# Supplementary material for: Origin of cosmological temperature
Source: arXiv:2005.05349 ancillary file (2020-05-11)
Supplement: Supplementary file 1 [file Calculations_for_Origin_of_cosmological_temperature.pdf]

# Calculations for *Origin of Cosmological Temperature*

Daniel Friedan

*New High Energy Theory Center and Department of Physics and Astronomy,  
Rutgers, The State University of New Jersey,  
Piscataway, New Jersey 08854-8019 U.S.A. and*

*Science Institute, The University of Iceland, Reykjavik, Iceland*

dfriedan@gmail.com      [www.physics.rutgers.edu/~friedan/](http://www.physics.rutgers.edu/~friedan/)

May 11, 2020

This note shows calculations for the paper *Origin of Cosmological Temperature*. The calculations are elementary. They are written out so that the details can be checked. The numerical calculations (mostly simple arithmetic) are shown in Appendix A. They were performed in a SageMath notebook that is included in the Supplemental Materials.

The Supplemental Materials — the SageMath notebook, renditions of it into html and pdf, and this note — are available at [https://cocalc.com/share/3c1ab84c375769c3460251d4f2bd43461c1211b5/Supplemental\\_material/](https://cocalc.com/share/3c1ab84c375769c3460251d4f2bd43461c1211b5/Supplemental_material/) and at [http://www.physics.rutgers.edu/pages/friedan/papers/2020/Origin/Supplemental\\_material/](http://www.physics.rutgers.edu/pages/friedan/papers/2020/Origin/Supplemental_material/).

To run the notebook, either install SageMath from [sagemath.org](http://sagemath.org) or create an account at [cocalc.com](http://cocalc.com) and upload the notebooks to run there. SageMath is a free open-source mathematics software system. Both free and paid accounts are available at [cocalc.com](http://cocalc.com). Paying for an account supports SageMath (see [reasons-for-purchasing-a-subscription](#)). Open-source mathematics software such as SageMath is essential for scientific research. Scientific results must be open to scrutiny. Closed-source mathematics software blocks scrutiny.

## Contents

|          |                                                         |           |
|----------|---------------------------------------------------------|-----------|
| <b>1</b> | <b>Classical action</b>                                 | <b>3</b>  |
| <b>2</b> | <b>Spin(4) symmetry</b>                                 | <b>3</b>  |
| 2.1      | Identify $S^3$ with $SU(2)$                             | 4         |
| 2.2      | Spin(4) acts as $SO(4)$ on space-time                   | 4         |
| 2.3      | $SO(4)$ -symmetric metric                               | 5         |
| 2.4      | $SU(2)$ scalar and gauge fields                         | 5         |
| 2.5      | Spin(4)-symmetric scalar and gauge fields               | 6         |
| <b>3</b> | <b>Classical action of the Spin(4)-symmetric fields</b> | <b>7</b>  |
| 3.1      | Ricci tensor                                            | 7         |
| 3.2      | Gravitational action                                    | 8         |
| 3.3      | Gauge field action                                      | 9         |
| 3.4      | Scalar field action                                     | 10        |
| 3.5      | Action in dimensionless variables                       | 10        |
| <b>4</b> | <b>Classical equations of motion</b>                    | <b>12</b> |

|          |                                                                          |    |
|----------|--------------------------------------------------------------------------|----|
| 4.1      | Gravitational equation of motion and energy-momentum tensors             | 12 |
| 4.2      | Gauge and scalar equations of motion                                     | 12 |
| 4.3      | Spin(4)-symmetric energy-momentum tensors                                | 13 |
| 4.4      | Spin(4)-symmetric gravitational equation of motion                       | 14 |
| 4.5      | Spin(4)-symmetric gauge and scalar equations of motion                   | 15 |
| <b>5</b> | <b>Numbers</b>                                                           | 16 |
| 5.1      | Fundamental constants                                                    | 16 |
| 5.2      | Standard Model coupling constants                                        | 17 |
| 5.3      | Gravitational and weak time scales $t_{\text{grav}}, t_W$                | 17 |
| 5.4      | The scalar field energy density $\mathcal{E}_0$                          | 17 |
| 5.5      | Seesaw time scale $t_I$                                                  | 17 |
| 5.6      | Seesaw ratio $\epsilon_w$                                                | 18 |
| 5.7      | Units of action for the two oscillators                                  | 18 |
| <b>6</b> | <b>Stability of <math>\phi = 0</math></b>                                | 18 |
| 6.1      | Dirac matrices and spinors on $S^3$                                      | 19 |
| 6.2      | Time-averaged stability                                                  | 19 |
| 6.3      | Spinor covariant derivative                                              | 20 |
| 6.4      | Dirac operator                                                           | 20 |
| 6.5      | Parity operator                                                          | 21 |
| 6.6      | Time-averaged stability (II)                                             | 22 |
| <b>7</b> | <b>Solution of the <math>b</math> oscillator by an elliptic function</b> | 22 |
| 7.1      | Reparametrize $T$ and $b$                                                | 22 |
| 7.2      | The Jacobi elliptic function $\text{cn}(z, k)$                           | 23 |
| 7.3      | Properties of the Jacobi elliptic functions                              | 23 |
| 7.4      | Complete elliptic integral of first kind $K(k), K'(k)$                   | 25 |
| 7.5      | $K(1/\sqrt{2})$                                                          | 25 |
| 7.6      | $\langle \text{cn}^2 \rangle$ for $k = 1/\sqrt{2}$                       | 26 |
| 7.7      | $\langle \text{cn}^2 \rangle$ for general $k$                            | 26 |
| <b>8</b> | <b>Cosmological temperature</b>                                          | 27 |
| <b>9</b> | <b>Solution of the <math>\hat{a}</math> oscillator</b>                   | 27 |
| 9.1      | Solution for $\hat{a}$ in co-moving time                                 | 27 |
| 9.2      | $\hat{a}_{\text{EW}}$                                                    | 29 |
| 9.3      | The function $u(z, k)$                                                   | 30 |
| 9.4      | Direct solution of the $\hat{a}$ oscillator by an elliptic function      | 31 |
| <b>A</b> | <b>Numerical calculations</b>                                            | 33 |
|          | <b>References</b>                                                        | 39 |

# 1 Classical action

Consider the classical equations of motion of the Standard Model combined with General Relativity, assuming

1. the only nonzero fields are
  - the space-time metric  $g_{\mu\nu}(x)$ ,
  - the SU(2) gauge field  $B_\mu(x) \in \mathfrak{su}(2)$ ,
  - the Higgs scalar field  $\phi(x) \in \mathbb{C}^2$ ,
2. space is the 3-sphere  $S^3$ , and
3. the universe is Spin(4)-symmetric.

The action (in units of  $\hbar$  with  $c = 1$ ) is

$$\begin{aligned}
\frac{1}{\hbar}S &= \frac{1}{\hbar}S_{\text{grav}} + \frac{1}{\hbar}S_{\text{gauge}} + \frac{1}{\hbar}S_{\text{scalar}} \\
\frac{1}{\hbar}S_{\text{grav}} &= \int \frac{1}{\hbar} \frac{R}{2\kappa} \sqrt{-g} d^4x \\
\frac{1}{\hbar}S_{\text{gauge}} &= \int \frac{1}{2g^2} \text{tr}(F_{\mu\nu}F^{\mu\nu}) \sqrt{-g} d^4x \\
\frac{1}{\hbar}S_{\text{scalar}} &= \int \left[ -D_\mu \phi^\dagger D^\mu \phi - \frac{1}{2} \lambda^2 \left( \phi^\dagger \phi - \frac{1}{2} v^2 \right)^2 \right] \sqrt{-g} d^4x
\end{aligned} \tag{1.1}$$

The gauge covariant derivative and curvature 2-form are

$$D_\mu \phi = (\partial_\mu + B_\mu) \phi \quad F_{\mu\nu} = [D_\mu, D_\nu] = \partial_\mu B_\nu - \partial_\nu B_\mu + [B_\mu, B_\nu] \tag{1.2}$$

## 2 Spin(4) symmetry

Space is the 3-sphere  $S^3$ . Space-time is  $I \times S^3$  where time  $I$  is a real interval. Use indices  $\mu, \nu$  for points  $x^\mu$  in space-time. Parametrize space-time by  $x = (x^0, \hat{x})$  with  $x^0 \in I$  and  $\hat{x}$  in the unit 3-sphere  $S^3$  in euclidean 4-space. Use indices  $j, k$  for euclidean 4-space.

$$\hat{x} \in S^3 \subset \mathbb{R}^4 \quad \hat{x} = (\hat{x}^1, \hat{x}^2, \hat{x}^3, \hat{x}^4) \quad \hat{x}_k \hat{x}^k = 1 \quad \hat{x}_k = \hat{x}^j \delta_{jk} \quad \hat{x}_k d\hat{x}^k = 0 \tag{2.1}$$

Spin(4) = SU(2)<sub>L</sub> × SU(2)<sub>R</sub> is the simply connected covering group of SO(4). Let  $\sigma_a$ ,  $a = 1, 2, 3$  be the Pauli matrices.

$$\sigma_a^\dagger = \sigma_a \quad \sigma_a \sigma_b = \delta_{ab} \mathbf{1} + \epsilon_{abc} i \sigma_c \quad \text{tr}(\sigma_a \sigma_b) = 2 \delta_{ab} \tag{2.2}$$

The anti-hermitian matrices  $i^{-1} \sigma_a$  form a basis for the Lie algebra  $\mathfrak{su}(2)$ . Use indices  $a, b, c$  for elements of  $\mathfrak{su}(2)$ .

## 2.1 Identify $S^3$ with $SU(2)$

Identify the unit 3-sphere  $S^3$  with the group  $SU(2)$  by

$$\hat{x} \longleftrightarrow g_{\hat{x}} = \hat{x}^4 \mathbf{1} + \hat{x}^a i^{-1} \sigma_a = \begin{pmatrix} \hat{x}^4 - i\hat{x}^3 & -i\hat{x}^1 - \hat{x}^2 \\ -i\hat{x}^1 + \hat{x}^2 & \hat{x}^4 + i\hat{x}^3 \end{pmatrix} \quad (2.3)$$

checking that

$$\begin{aligned} (g_{\hat{x}})^\dagger g_{\hat{x}} &= (\hat{x}^4 \mathbf{1} - \hat{x}^a i^{-1} \sigma_a)(\hat{x}^4 \mathbf{1} + \hat{x}^b i^{-1} \sigma_b) = (\hat{x}^4)^2 \mathbf{1} + \hat{x}^a \hat{x}^b \sigma_a \sigma_b = \delta_{jk} \hat{x}^j \hat{x}^k \mathbf{1} = \mathbf{1} \\ \det g_{\hat{x}} &= |\hat{x}^4 - i\hat{x}^3|^2 + |-i\hat{x}^1 - \hat{x}^2|^2 = \delta_{jk} \hat{x}^j \hat{x}^k = 1 \end{aligned} \quad (2.4)$$

The north-pole  $\hat{N}$  in  $S^3$  is identified with the identity element  $\mathbf{1}$  in  $SU(2)$

$$\hat{N} = (0, 0, 0, 1) \quad g_{\hat{N}} = \mathbf{1} \quad (2.5)$$

The tangent space to  $S^3$  at  $\hat{N}$  is identified with the Lie algebra  $\mathfrak{su}(2)$

$$dg_{\hat{x}}(\hat{N}) = d\hat{x}^a i^{-1} \sigma_a \quad (2.6)$$

The identity

$$\text{tr}(g_{\hat{x}}^{-1} g_{\hat{y}}) = \text{tr}(g_{\hat{x}}^\dagger g_{\hat{y}}) = \text{tr}((\hat{x}^4)^2 \mathbf{1} + \hat{x}^a \hat{x}^b \sigma_a \sigma_b) = 2\delta_{jk} \hat{x}^j \hat{y}^k \quad (2.7)$$

identifies the metric of the unit 3-sphere with the Killing form on  $SU(2)$

$$ds_{S^3}^2 = \delta_{jk} d\hat{x}^j d\hat{y}^k = \frac{1}{2} \text{tr}(dg_{\hat{x}}^{-1} dg_{\hat{y}}) \quad (2.8)$$

At the north-pole the metric of the unit 3-sphere is

$$ds_{S^3}^2(\hat{N}) = \delta_{ab} d\hat{x}^a d\hat{x}^b \quad (2.9)$$

The metric volume element of the unit 3-sphere is

$$d^3 \hat{x} = d^4 x \delta(r-1) \quad r^2 = x_k x^k \quad \int_{S^3} d^3 \hat{x} = 2\pi^2 \quad (2.10)$$

## 2.2 $\text{Spin}(4)$ acts as $\text{SO}(4)$ on space-time

An element  $U = (g_L, g_R)$  in  $\text{Spin}(4) = SU(2)_L \times SU(2)_R$  acts on  $S^3$  by

$$U = (g_L, g_R) \quad g_{\hat{x}} \mapsto g_L g_{\hat{x}} g_R^{-1} \quad \hat{x} \mapsto U\hat{x} \quad g_{U\hat{x}} = g_L g_{\hat{x}} g_R^{-1} \quad (2.11)$$

$\hat{x} \mapsto U\hat{x}$  is an  $\text{SO}(4)$  rotation because the identity (2.7) implies

$$\delta_{jk}(U\hat{x})^j (U\hat{y})^k = \delta_{jk} \hat{x}^j \hat{y}^k \quad (2.12)$$

The map  $\text{Spin}(4) \rightarrow \text{SO}(4)$  is 2-to-1 because  $(g_L, g_R) = (-1, -1)$  acts as the identity.  $\text{Spin}(4)$  acts on space-time by rotating space independent of time

$$x \mapsto Ux \quad (x^0, \hat{x}) \mapsto (x^0, U\hat{x}) \quad (2.13)$$

$\text{Spin}(4)$  takes the north-pole  $\hat{N}$  to any other point in  $S^3$  so a  $\text{Spin}(4)$ -symmetric field is completely determined by its value at  $\hat{N}$ . The value at  $\hat{N}$  must be invariant under the little group at  $\hat{N}$ , the subgroup that takes  $\hat{N}$  to itself,  $g_L \mathbf{1} g_R^{-1} = \mathbf{1}$ , which is the diagonal subgroup  $SU(2)_\Delta = \{(g_L, g_L)\}$ . The little group acts on the tangent space to  $S^3$  at  $\hat{N}$  as the adjoint action of  $SU(2)$  on the Lie algebra  $\mathfrak{su}(2)$ .

$$\text{at } \hat{x} = \hat{N}, \quad d(g_L g_{\hat{x}} g_L^{-1}) = d\hat{x}^a g_L (i^{-1} \sigma_a) g_L^{-1} \quad (2.14)$$

### 2.3 SO(4)-symmetric metric

If  $g_{\mu\nu}(x)$  is an SO(4)-invariant space-time metric, its value at the north-pole is

$$\begin{aligned} g_{\mu\nu}(\hat{N})dx^\mu dx^\nu &= g_{00}(x^0)(dx^0)^2 + g_{0a}(x^0)(dx^0 d\hat{x}^a + d\hat{x}^a dx^0) + g_{ab}(x^0)d\hat{x}^a d\hat{x}^b \\ &= -F_1(x^0)^2(dx^0)^2 + F_2(x^0)^2\delta_{ab}d\hat{x}^a d\hat{x}^b \end{aligned} \quad (2.15)$$

The off-diagonal term  $g_{0a}(x^0) = 0$  because it must be an element of  $\mathfrak{su}(2)$  invariant under the adjoint action. The only such element is 0. The spatial metric  $g_{ab}(x^0)$  is an invariant positive bilinear form on  $\mathfrak{su}(2)$  therefore a multiple of the Killing form. So the general SO(4)-invariant space-time metric has the form

$$g_{\mu\nu}(x)dx^\mu dx^\nu = -F_1(x^0)^2(dx^0)^2 + F_2(x^0)^2 ds_{S^3}^2 \quad (2.16)$$

where  $ds_{S^3}^2$  is the metric of the unit 3-sphere.

Make a reparametrization of time  $x^0 \rightarrow T(x^0)$  such that

$$\frac{dT}{dx^0} = \frac{F_1(x^0)}{F_2(x^0)} \quad (2.17)$$

and define  $a(T) = F_2(x^0)$ . The space-time metric is now in the conformally flat form

$$g_{\mu\nu}(x)dx^\mu dx^\nu = a(T)^2 (-dT^2 + ds_{S^3}^2) \quad (2.18)$$

To see that this metric is conformally flat, Wick rotate to imaginary time  $\tau = iT$ . Then

$$\begin{aligned} g_{\mu\nu}(x)dx^\mu dx^\nu &= a^2 (d\tau^2 + ds_{S^3}^2) \\ &= a^2 r^{-2} (dr^2 + r^2 ds_{S^3}^2) & r = e^\tau \\ &= a^2 r^{-2} \delta_{jk} dx^j dx^k & r^2 = x_k x^k \end{aligned} \quad (2.19)$$

so  $g_{\mu\nu}(x)$  is conformal to the flat euclidean metric on  $\mathbb{R}^4$  with conformal factor  $a^2 r^{-2}$ .

The metric volume element is

$$\sqrt{-g} d^4 x = a^4 dT d^3 \hat{x} \quad (2.20)$$

where  $d^3 \hat{x}$  is the volume element of the unit 3-sphere.

### 2.4 SU(2) scalar and gauge fields

All SU(2) vector bundles over  $S^3$  are trivial bundles, so the fundamental SU(2) vector bundle on space-time can be identified with the product space  $(I \times S^3) \times \mathbb{C}^2$ . An SU(2) scalar field  $\phi(x)$  is a function on space-time whose value at each point is a complex 2-vector

$$\phi(x) = \begin{pmatrix} \phi^1 \\ \phi^2 \end{pmatrix} (x) \quad (2.21)$$

i.e., a section of the fundamental SU(2) vector bundle.

An SU(2) gauge field is an  $\mathfrak{su}(2)$ -valued 1-form  $B(x)$  on space-time. The gauge covariant derivative is

$$\begin{aligned} D &= d + B & D &= dx^\mu D_\mu & D_\mu &= \partial_\mu + B_\mu(x) \\ B &= dx^\mu B_\mu(x) & B_\mu(x) &= B_\mu^a(x) i^{-1} \sigma_a & D_\mu \phi(x) &= \partial_\mu \phi(x) + B_\mu(x) \phi(x) \end{aligned} \quad (2.22)$$

The curvature 2-form is

$$\begin{aligned} F &= D \wedge D = dB + B \wedge B \\ F &= \frac{1}{2} dx^\mu \wedge dx^\nu F_{\mu\nu} & F_{\mu\nu} &= \partial_\mu B_\nu - \partial_\nu B_\mu + [B_\mu, B_\nu] \end{aligned} \quad (2.23)$$

## 2.5 Spin(4)-symmetric scalar and gauge fields

Let  $\text{Spin}(4) = \text{SU}(2)_L \times \text{SU}(2)_R$  act on the fundamental vector bundle by

$$x = (T, g_{\hat{x}}) \quad U = (g_L, g_R) \quad \phi(x) \mapsto g_L^{-1} \phi(Ux) = g_L^{-1} \phi(T, g_L g_{\hat{x}} g_R^{-1}) \quad (2.24)$$

so  $\text{Spin}(4)$  acts on gauge fields by

$$B(x) \mapsto g_L^{-1} B(Ux) g_L \quad dx^\mu B_\mu(x) \mapsto d(Ux)^\mu g_L^{-1} B_\mu(Ux) g_L \quad (2.25)$$

$\text{Spin}(4)$ -symmetric fields are left unchanged

$$\phi(x) = g_L^{-1} \phi(Ux) \quad B(x) = g_L^{-1} B(Ux) g_L \quad (2.26)$$

For an invariant scalar field  $\phi(T, \hat{x})$ , the value at  $\hat{x} = \hat{N}$  is a vector  $\phi(T, \hat{N}) \in \mathbb{C}^2$ . An element  $(g_L, g_L)$  of the little group takes  $\hat{N}$  to itself so

$$\phi(T, \hat{N}) \rightarrow g_L^{-1} \phi(T, \hat{N}) \quad (2.27)$$

Invariance under the little group means that  $\phi(T, \hat{N})$  is invariant under every  $g_L \in \text{SU}(2)$ . The only such vector is 0. So  $\phi(x) = 0$ .

For an invariant gauge field  $B(x)$ , the value at  $\hat{N}$  is a 1-form

$$B(T, \hat{N}) = dT B_0^a(T, \hat{N}) i^{-1} \sigma_a + d\hat{x}^b B_b^a(T, \hat{N}) i^{-1} \sigma_a \quad (2.28)$$

Invariance under the little group requires  $B_0^a$  to be an element of  $\mathfrak{su}(2)$  invariant under the adjoint  $\text{SU}(2)$  action. The only invariant element of  $\mathfrak{su}(2)$  is 0. So  $B_0^a = 0$ .  $B_b^a$  must be an invariant linear map from  $\mathfrak{su}(2)$  to itself so must be proportional to the identity. Write this proportionality

$$B_b^a(T, \hat{N}) = [1 + b(T)] \left( -\frac{1}{2} \delta_b^a \right) \quad (2.29)$$

Define the  $\mathfrak{su}(2)$ -valued 1-form on  $S^3$

$$\gamma(\hat{x}) = -\frac{1}{2} (dg_{\hat{x}}) g_{\hat{x}}^{-1} = \frac{1}{2} g_{\hat{x}} dg_{\hat{x}}^\dagger \quad (2.30)$$

$\gamma(\hat{x})$  is  $\text{Spin}(4)$ -symmetric.

$$g_L^{-1} \gamma(U\hat{x}) g_L = -g_L^{-1} \frac{1}{2} d(g_L g_{\hat{x}} g_R^{-1}) (g_L g_{\hat{x}} g_R^{-1})^{-1} g_L = \gamma(\hat{x}) \quad (2.31)$$

Its value at the north-pole is a multiple of the identity matrix.

$$\gamma(\hat{N}) = -\frac{1}{2} d\hat{x}^a i^{-1} \sigma_a = d\hat{x}^b \left( -\frac{1}{2} \delta_b^a \right) i^{-1} \sigma_a \quad (2.32)$$

so at the north-pole

$$B(T, \hat{N}) = [1 + b(T)] \gamma(\hat{N}) \quad (2.33)$$

so by  $\text{Spin}(4)$ -symmetry the identity holds everywhere

$$B(T, \hat{x}) = [1 + b(T)] \gamma(\hat{x}) \quad (2.34)$$

### 3 Classical action of the Spin(4)-symmetric fields

#### 3.1 Ricci tensor

For the conformally flat space-time metric (2.18)

$$g_{\mu\nu}(x)dx^\mu dx^\nu = a(T)^2 (-dT^2 + ds_{S^3}^2) \quad (3.1)$$

now calculate the Ricci tensor  $R_{\mu\nu}$ . The result will be

$$R_{\mu\nu}dx^\mu dx^\nu = [-3a^{-1}\partial_T^2 a + 3a^{-2}(\partial_T a)^2] dT^2 + [a^{-1}\partial_T^2 a + a^{-2}(\partial_T a)^2 + 2] ds_{S^3}^2 \quad (3.2)$$

from which the scalar curvature is

$$\begin{aligned} R = g^{\mu\nu} R_{\mu\nu} &= -a^{-2} [-3a^{-1}\partial_T^2 a + 3a^{-2}(\partial_T a)^2] + 3a^{-2} [a^{-1}\partial_T^2 a + a^{-2}(\partial_T a)^2 + 2] \\ &= 6a^{-2} (a^{-1}\partial_T^2 a + 1) \end{aligned} \quad (3.3)$$

and the Einstein tensor is

$$\begin{aligned} G_{\mu\nu} &= R_{\mu\nu} - \frac{1}{2} R g_{\mu\nu} \\ G_{\mu\nu}dx^\mu dx^\nu &= [-3a^{-1}\partial_T^2 a + 3a^{-2}(\partial_T a)^2] dT^2 + [a^{-1}\partial_T^2 a + a^{-2}(\partial_T a)^2 + 2] ds_{S^3}^2 \\ &\quad - \frac{1}{2} 6a^{-2} (a^{-1}\partial_T^2 a + 1) a^2 (-dT^2 + ds_{S^3}^2) \\ &= [3a^{-2}(\partial_T a)^2 + 3] dT^2 + [a^{-2}(\partial_T a)^2 - 2a^{-1}\partial_T^2 a - 1] ds_{S^3}^2 \end{aligned} \quad (3.4)$$

To calculate the Ricci tensor, first analytically continue to imaginary time  $\tau = iT$ ,

$$g_{\mu\nu}(x)dx^\mu dx^\nu = a^2 (d\tau^2 + ds_{S^3}^2) \quad \tau = iT \quad (3.5)$$

then change space-time coordinates from  $(\tau, \hat{x}^k)$  to  $x^k = r\hat{x}^k$ ,  $r = e^\tau$ ,

$$\begin{aligned} x^k &= r\hat{x}^k \quad r = e^\tau \\ g_{\mu\nu}(x)dx^\mu dx^\nu &= g_{jk}dx^j dx^k = a^2 r^{-2} (dr^2 + r^2 ds_{S^3}^2) = a^2 r^{-2} \delta_{jk} dx^j dx^k \\ g_{jk} &= e^{2f} \delta_{jk} \quad e^{2f} = a^2 r^{-2} \end{aligned} \quad (3.6)$$

The metric covariant derivative of a vector field  $v^i(x)$  is

$$\begin{aligned} \nabla_k v^i &= \partial_k v^i + \Gamma_{jk}^i v^j \\ \Gamma_{jk}^i &= \frac{1}{2} g^{im} (\partial_j g_{km} + \partial_k g_{jm} - \partial_i g_{jk}) = \partial_j f \delta_k^i + \partial_k f \delta_j^i - \partial^i f \delta_{jk} \end{aligned} \quad (3.7)$$

using  $\delta_{ij}$  to raise and lower indices. The metric curvature tensor is

$$\begin{aligned} (\nabla_j \nabla_k - \nabla_k \nabla_j) v^m &= R_{ijk}^m v^i \\ R_{ijk}^m &= \partial_j \Gamma_{ki}^m - \partial_k \Gamma_{ji}^m + \Gamma_{nj}^m \Gamma_{ik}^n - \Gamma_{nk}^m \Gamma_{ij}^n \end{aligned} \quad (3.8)$$

The Ricci tensor is

$$R_{ik} = R_{ijk}^j = \partial_j \Gamma_{ki}^j - \partial_k \Gamma_{ji}^j + \Gamma_{nj}^j \Gamma_{ik}^n - \Gamma_{nk}^j \Gamma_{ij}^n \quad (3.9)$$

Substituting,

$$\begin{aligned}
R_{ik} &= \partial_j (\partial_k f \delta_i^j + \partial_i f \delta_k^j - \partial^j f \delta_{ki}) - \partial_k (\partial_j f \delta_i^j + \partial_i f \delta_j^j - \partial^j f \delta_{ji}) \\
&\quad + (\partial_n f \delta_j^j + \partial_j f \delta_n^j - \partial^j f \delta_{nj}) (\partial_i f \delta_k^n + \partial_k f \delta_i^n - \partial^n f \delta_{ik}) \\
&\quad - (\partial_n f \delta_k^j + \partial_k f \delta_n^j - \partial^j f \delta_{nk}) (\partial_i f \delta_j^n + \partial_j f \delta_i^n - \partial^n f \delta_{ij}) \\
&= -2\partial_i \partial_k f - \partial^j \partial_j f \delta_{ik} + 2\partial_i f \partial_k f - 2\partial_j f \partial^j f \delta_{ik}
\end{aligned} \tag{3.10}$$

Now use that  $f$  depends only on  $r = e^\tau$

$$\begin{aligned}
\partial_i \tau &= r^{-1} \hat{x}_i & \partial_i \partial_k \tau &= r^{-2} (\delta_{ik} - 2\hat{x}_i \hat{x}_k) \\
\partial_i f &= \partial_i \tau \partial_\tau f = r^{-1} \hat{x}_i \partial_\tau f \\
\partial_i \partial_k f &= \partial_i \partial_k \tau \partial_\tau f + \partial_i \tau \partial_k \tau \partial_\tau^2 f = r^{-2} [(\delta_{ik} - 2\hat{x}_i \hat{x}_k) \partial_\tau f + \hat{x}_i \hat{x}_k \partial_\tau^2 f] \\
\partial_j \partial^j f &= r^{-2} (2\partial_\tau f + \partial_\tau^2 f)
\end{aligned} \tag{3.11}$$

$$\begin{aligned}
R_{ik} &= -2r^{-2} [(\delta_{ik} - 2\hat{x}_i \hat{x}_k) \partial_\tau f + \hat{x}_i \hat{x}_k \partial_\tau^2 f] - r^{-2} (2\partial_\tau f + \partial_\tau^2 f) \delta_{ik} \\
&\quad + 2r^{-2} \hat{x}_i \hat{x}_k (\partial_\tau f)^2 - 2r^{-2} (\partial_\tau f)^2 \delta_{ik} \\
&= r^{-2} \hat{x}_i \hat{x}_k [4\partial_\tau f - 2\partial_\tau^2 f + 2(\partial_\tau f)^2] + r^{-2} \delta_{ik} [-4\partial_\tau f - \partial_\tau^2 f - 2(\partial_\tau f)^2] \\
&= r^{-2} \hat{x}_i \hat{x}_k (-3\partial_\tau^2 f) + r^{-2} (\delta_{ik} - \hat{x}_i \hat{x}_k) [-4\partial_\tau f - \partial_\tau^2 f - 2(\partial_\tau f)^2]
\end{aligned} \tag{3.12}$$

Substitute

$$f = \ln a - \tau \quad \partial_\tau f = a^{-1} \partial_\tau a - 1 \quad \partial_\tau^2 f = a^{-1} \partial_\tau^2 a - a^{-2} (\partial_\tau a)^2 \tag{3.13}$$

to get

$$\begin{aligned}
R_{ik} &= r^{-2} \hat{x}_i \hat{x}_k [-3a^{-1} \partial_\tau^2 a + 3a^{-2} (\partial_\tau a)^2] \\
&\quad + r^{-2} (\delta_{ik} - \hat{x}_i \hat{x}_k) [-4a^{-1} \partial_\tau a + 4 - a^{-1} \partial_\tau^2 a + a^{-2} (\partial_\tau a)^2 \\
&\quad \quad - 2(a^{-1} \partial_\tau a - 1)^2] \\
&= r^{-2} \hat{x}_i \hat{x}_k [-3a^{-1} \partial_\tau^2 a + 3a^{-2} (\partial_\tau a)^2] \\
&\quad + r^{-2} (\delta_{ik} - \hat{x}_i \hat{x}_k) [2 - a^{-1} \partial_\tau^2 a - a^{-2} (\partial_\tau a)^2]
\end{aligned} \tag{3.14}$$

Finally return to real time  $T$ ,

$$r^{-2} \hat{x}_i \hat{x}_k dx^i dx^k = d\tau^2 = -dT^2 \quad r^{-2} (\delta_{ik} - \hat{x}_i \hat{x}_k) dx^i dx^k = ds_{S^3}^2 \tag{3.15}$$

to get the Ricci tensor formula

$$\begin{aligned}
R_{\mu\nu} dx^\mu dx^\nu &= R_{ik} dx^i dx^k \\
&= [-3a^{-1} \partial_T^2 a + 3a^{-2} (\partial_T a)^2] dT^2 + [a^{-1} \partial_T^2 a + a^{-2} (\partial_T a)^2 + 2] ds_{S^3}^2
\end{aligned} \tag{3.16}$$

### 3.2 Gravitational action

Using formula (3.3) for the scalar curvature, the gravitational action is

$$\begin{aligned}
\frac{1}{\hbar} S_{\text{grav}} &= \int \frac{1}{2\kappa\hbar} R \sqrt{-g} d^4x \\
&= \int \frac{1}{2\kappa\hbar} 6a^{-2} (a^{-1} \partial_T^2 a + 1) a^4 dT \int_{S^3} d^3\hat{x} \\
&= \frac{12\pi^2}{\kappa\hbar} \int \frac{1}{2} (a \partial_T^2 a + a^2) dT
\end{aligned} \tag{3.17}$$

Integrating by parts and discarding the boundary terms gives

$$\frac{1}{\hbar} S_{\text{grav}} = \frac{12\pi^2}{\kappa\hbar} \int \frac{1}{2} [-(\partial_T a)^2 + a^2] dT \quad (3.18)$$

### 3.3 Gauge field action

To find the gauge field action of the Spin(4)-symmetric gauge field (2.34)

$$\frac{1}{\hbar} S_{\text{gauge}} = \int \frac{1}{2g^2} \text{tr}(F_{\mu\nu} F^{\mu\nu}) \sqrt{-g} d^4x \quad B(T, \hat{x}) = [1 + b(T)] \gamma(\hat{x}) \quad (3.19)$$

in the SO(4)-symmetric conformally flat metric (2.18)

$$g_{\mu\nu}(x) dx^\mu dx^\nu = a(T)^2 (-dT^2 + ds_{S^3}^2) \quad (3.20)$$

first calculate the curvature 2-form

$$\begin{aligned} dB &= (\partial_T b) dT \wedge \gamma + (1 + b) d\gamma \\ F &= dB + B \wedge B = (\partial_T b) dT \wedge \gamma + (1 + b) d\gamma + (1 + b)^2 \gamma \wedge \gamma \end{aligned} \quad (3.21)$$

then use the identity

$$\begin{aligned} d\gamma &= d \left[ -\frac{1}{2} (dg_{\hat{x}}) g_{\hat{x}}^{-1} \right] = \frac{1}{2} (dg_{\hat{x}}) \wedge d(g_{\hat{x}}^{-1}) = -\frac{1}{2} (dg_{\hat{x}}) \wedge g_{\hat{x}}^{-1} (dg_{\hat{x}}) g_{\hat{x}}^{-1} \\ &= -2\gamma \wedge \gamma \end{aligned} \quad (3.22)$$

to get

$$F = (\partial_T b) dT \wedge \gamma + (b^2 - 1) \gamma \wedge \gamma \quad (3.23)$$

Next find the components  $F_{\mu\nu}(T, \hat{N})$  at the north-pole.

$$\begin{aligned} F(T, \hat{N}) &= \frac{1}{2} F_{\mu\nu} dx^\mu \wedge dx^\nu = F_{0a} dT \wedge d\hat{x}^a + \frac{1}{2} F_{ab} d\hat{x}^a \wedge d\hat{x}^b \\ \gamma \wedge \gamma(\hat{N}) &= \left( -\frac{1}{2} d\hat{x}^a i^{-1} \sigma_a \right) \wedge \left( -\frac{1}{2} d\hat{x}^b i^{-1} \sigma_b \right) = \frac{1}{4} d\hat{x}^a \wedge d\hat{x}^b \epsilon_{abc} i^{-1} \sigma_c \\ F(T, \hat{N}) &= (\partial_T b) dT \wedge \left( -\frac{1}{2} d\hat{x}^a i^{-1} \sigma_a \right) + (b^2 - 1) \frac{1}{4} d\hat{x}^a \wedge d\hat{x}^b \epsilon_{abc} i^{-1} \sigma_c \end{aligned} \quad (3.24)$$

$$F_{0a}(T, \hat{N}) = -\frac{1}{2} \partial_T b i^{-1} \sigma_a \quad F_{ab}(T, \hat{N}) = \frac{1}{2} (b^2 - 1) \epsilon_{abc} i^{-1} \sigma_c$$

Then evaluate  $\text{tr}(F_{\mu\nu} F^{\mu\nu})$  at the north-pole.

$$\begin{aligned} \text{tr}(F_{\mu\nu} F^{\mu\nu})(T, \hat{N}) &= a^{-4} \text{tr} \left( -2F_{0a} F_{0a'} \delta^{aa'} + F_{ab} F_{a'b'} \delta^{aa'} \delta^{bb'} \right) \\ &= a^{-4} \text{tr} \left( \frac{1}{2} (\partial_T b)^2 \delta^{aa'} \sigma_a \sigma_{a'} - \frac{1}{4} (b^2 - 1)^2 \epsilon_{abc} \epsilon_{a'b'c'} \delta^{aa'} \delta^{bb'} \sigma_c \sigma_{c'} \right) \\ &= 3a^{-4} [(\partial_T b)^2 - (b^2 - 1)^2] \end{aligned} \quad (3.25)$$

This holds everywhere in space-time because  $\text{tr}(F_{\mu\nu} F^{\mu\nu})$  is a Spin(4)-invariant function.

$$\text{tr}(F_{\mu\nu} F^{\mu\nu}) = 3a^{-4} [(\partial_T b)^2 - (b^2 - 1)^2] \quad (3.26)$$

So the gauge field action is

$$\begin{aligned}
\frac{1}{\hbar} S_{\text{gauge}} &= \int \frac{1}{2g^2} \text{tr}(F_{\mu\nu} F^{\mu\nu}) \sqrt{-g} d^4x \\
&= \int \frac{1}{2g^2} 3a^{-4} [(\partial_T b)^2 - (b^2 - 1)^2] a^4 dT \int_{S^3} d^3\hat{x} \\
&= \frac{6\pi^2}{g^2} \int \frac{1}{2} [(\partial_T b)^2 - (b^2 - 1)^2] dT
\end{aligned} \tag{3.27}$$

### 3.4 Scalar field action

The action of the Spin(4)-symmetric scalar field  $\phi = 0$  is

$$\begin{aligned}
\frac{1}{\hbar} S_{\text{scalar}} &= \int \left[ -D_\mu \phi^\dagger D^\mu \phi - \frac{1}{2} \lambda^2 \left( \phi^\dagger \phi - \frac{1}{2} v^2 \right)^2 \right] \sqrt{-g} d^4x \\
&= \int \left( -\frac{1}{8} \lambda^2 v^4 \right) a^4 dT \int_{S^3} d^3\hat{x} \\
&= 2\pi^2 \int \left( -\frac{1}{8} \lambda^2 v^4 \right) a^4 dT \\
&= 2\pi^2 \int \left( -\frac{1}{\hbar} \mathcal{E}_0 \right) a^4 dT \quad \frac{1}{\hbar} \mathcal{E}_0 = \frac{1}{8} \lambda^2 v^4
\end{aligned} \tag{3.28}$$

### 3.5 Action in dimensionless variables

The sum of the gravitational action (3.18) and the scalar action (3.28) is

$$\begin{aligned}
\frac{1}{\hbar} S_{\text{grav}} + \frac{1}{\hbar} S_{\text{scalar}} &= \frac{12\pi^2}{\kappa\hbar} \int \frac{1}{2} [-(\partial_T a)^2 + a^2] dT + 2\pi^2 \int \left( -\frac{1}{\hbar} \mathcal{E}_0 \right) a^4 dT \\
&= \frac{12\pi^2}{\kappa\hbar} \int \frac{1}{2} \left[ -(\partial_T a)^2 + a^2 - \frac{\kappa\mathcal{E}_0}{3} a^4 \right] dT
\end{aligned} \tag{3.29}$$

where

$$\frac{1}{\hbar} \mathcal{E}_0 = \frac{1}{8} \lambda^2 v^4 \tag{3.30}$$

Change variable

$$a = t_I \hat{a} \quad \frac{1}{\hbar} S_{\text{grav}} + \frac{1}{\hbar} S_{\text{scalar}} = \frac{12\pi^2 t_I^2}{\kappa\hbar} \int \frac{1}{2} \left[ -(\partial_T \hat{a})^2 + \hat{a}^2 - \frac{\kappa\mathcal{E}_0 t_I^2}{3} \hat{a}^4 \right] dT \tag{3.31}$$

Choose  $t_I$  so that

$$\frac{\kappa\mathcal{E}_0 t_I^2}{3} = 1 \quad t_I^2 = \frac{3}{\kappa\mathcal{E}_0} = \frac{24}{\kappa\hbar\lambda^2 v^4} \tag{3.32}$$

Then

$$\frac{1}{\hbar} S_{\text{grav}} + \frac{1}{\hbar} S_{\text{scalar}} = -\frac{12\pi^2 t_I^2}{\kappa\hbar} \int \left[ \frac{1}{2} (\partial_T \hat{a})^2 - \frac{1}{2} (\hat{a}^2 - \hat{a}^4) \right] dT \tag{3.33}$$

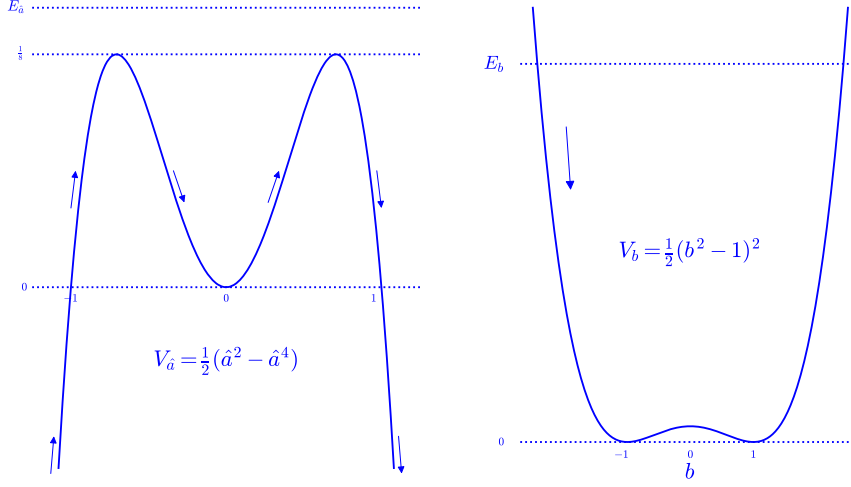

Figure 1: The anharmonic potentials. The energies  $E_{\hat{a}}$  and  $E_{\hat{b}}$  are not to scale.

Adding the gauge action (3.27), the total action is

$$\begin{aligned}
\frac{1}{\hbar}S &= \frac{1}{\hbar}S_{\text{grav}} + \frac{1}{\hbar}S_{\text{scalar}} + \frac{1}{\hbar}S_{\text{gauge}} \\
&= -\frac{12\pi^2 t_1^2}{\kappa\hbar} \int \left[ \frac{1}{2}(\partial_T \hat{a})^2 - \frac{1}{2}(\hat{a}^2 - \hat{a}^4) \right] dT \\
&\quad + \frac{6\pi^2}{g^2} \int \left[ \frac{1}{2}(\partial_T b)^2 - \frac{1}{2}(b^2 - 1)^2 \right] dT \\
&= \frac{6\pi^2}{g^2} \int \left( -\frac{g^2}{6\pi^2} \frac{12\pi^2 t_1^2}{\kappa\hbar} \left[ \frac{1}{2}(\partial_T \hat{a})^2 - \frac{1}{2}(\hat{a}^2 - \hat{a}^4) \right] \right. \\
&\quad \left. + \left[ \frac{1}{2}(\partial_T b)^2 - \frac{1}{2}(b^2 - 1)^2 \right] \right) dT
\end{aligned} \tag{3.34}$$

which is

$$\begin{aligned}
\frac{1}{\hbar}S &= \frac{6\pi^2}{g^2} \int \left( -\epsilon_w^{-4} \left[ \frac{1}{2}(\partial_T \hat{a})^2 - V_{\hat{a}}(\hat{a}) \right] + \left[ \frac{1}{2}(\partial_T b)^2 - V_b(b) \right] \right) dT \\
\epsilon_w^{-4} &= \frac{2g^2 t_1^2}{\kappa\hbar} \quad V_{\hat{a}}(\hat{a}) = \frac{1}{2}(\hat{a}^2 - \hat{a}^4) \quad V_b(b) = \frac{1}{2}(b^2 - 1)^2
\end{aligned} \tag{3.35}$$

The potentials are graphed in Figure 1.

## 4 Classical equations of motion

### 4.1 Gravitational equation of motion and energy-momentum tensors

Vary the action (1.1) with respect to a variation of the metric  $\delta g_{\mu\nu} = h_{\mu\nu}$ .

$$\begin{aligned}\delta S_{\text{grav}} &= \int h^{\mu\nu} \frac{1}{2\kappa} (-G_{\mu\nu}) \sqrt{-g} d^4x \\ &= \int h^{\mu\nu} \frac{1}{2\kappa} (-R_{\mu\nu} + \frac{1}{2} R g_{\mu\nu}) \sqrt{-g} d^4x\end{aligned}\quad (4.1)$$

$$\begin{aligned}\delta S_{\text{gauge}} &= \int h^{\mu\nu} \frac{1}{2} T_{\mu\nu}^{\text{gauge}} \sqrt{-g} d^4x \\ &= \int h^{\mu\nu} \frac{\hbar}{2g^2} \text{tr} \left( -2F_{\mu\sigma} F_{\nu}^{\sigma} + \frac{1}{2} g_{\mu\nu} F_{\rho\sigma} F^{\rho\sigma} \right) \sqrt{-g} d^4x\end{aligned}\quad (4.2)$$

$$\begin{aligned}\delta S_{\text{scalar}} &= \int h^{\mu\nu} \frac{1}{2} T_{\mu\nu}^{\text{scalar}} \sqrt{-g} d^4x \\ &= \int h^{\mu\nu} \hbar \left[ D_{\mu} \phi^{\dagger} D_{\nu} \phi - \frac{1}{2} g_{\mu\nu} D_{\sigma} \phi^{\dagger} D^{\sigma} \phi - \frac{1}{2} g_{\mu\nu} \frac{1}{2} \lambda^2 \left( \phi^{\dagger} \phi - \frac{1}{2} v^2 \right)^2 \right] \sqrt{-g} d^4x\end{aligned}\quad (4.3)$$

The gravitational equation of motion  $\delta S / \delta g_{\mu\nu} = 0$  is

$$-G_{\mu\nu} + \kappa T_{\mu\nu}^{\text{gauge}} + \kappa T_{\mu\nu}^{\text{scalar}} = 0 \quad (4.4)$$

where the energy-momentum tensors are

$$T_{\mu\nu}^{\text{gauge}} = \frac{\hbar}{g^2} \text{tr} \left( -2F_{\mu\sigma} F_{\nu}^{\sigma} + \frac{1}{2} g_{\mu\nu} F_{\rho\sigma} F^{\rho\sigma} \right) \quad (4.5)$$

$$T_{\mu\nu}^{\text{scalar}} = \hbar \left[ 2D_{\mu} \phi^{\dagger} D_{\nu} \phi - g_{\mu\nu} D_{\sigma} \phi^{\dagger} D^{\sigma} \phi - g_{\mu\nu} \frac{1}{2} \lambda^2 \left( \phi^{\dagger} \phi - \frac{1}{2} v^2 \right)^2 \right] \quad (4.6)$$

### 4.2 Gauge and scalar equations of motion

Vary the action with respect to a variation of the gauge field  $\delta B_{\mu}(x)$ .

$$\begin{aligned}\delta S_{\text{gauge}} &= \frac{\hbar}{2g^2} \int \text{tr} [4(D_{\mu} \delta B_{\nu}) F^{\mu\nu}] \sqrt{-g} d^4x \\ &= \hbar \int \text{tr} \left[ \delta B_{\mu} \left( \frac{2}{g^2} D_{\nu} F^{\mu\nu} \right) \right] \sqrt{-g} d^4x \\ \delta S_{\text{scalar}} &= \hbar \int \left[ -(\delta B_{\mu} \phi)^{\dagger} D^{\mu} \phi - D_{\mu} \phi^{\dagger} \delta B^{\mu} \phi \right] \sqrt{-g} d^4x \\ &= \hbar \int \left[ \phi^{\dagger} \delta B_{\mu} D^{\mu} \phi - D_{\mu} \phi^{\dagger} \delta B^{\mu} \phi \right] \sqrt{-g} d^4x \\ &= \hbar \int \text{tr} \left[ \delta B_{\mu} \left( D^{\mu} \phi \phi^{\dagger} - \phi D^{\mu} \phi^{\dagger} \right) \right] \sqrt{-g} d^4x\end{aligned}\quad (4.7)$$

So the gauge field equation of motion is

$$\frac{1}{2} D^{\nu} F_{\mu\nu} + \frac{g^2}{4} \left( D_{\mu} \phi \phi^{\dagger} - \phi D_{\mu} \phi^{\dagger} \right) = 0 \quad (4.8)$$

Vary the scalar field by  $\delta\phi$

$$\begin{aligned}
\delta S_{\text{scalar}} &= \hbar \int \left[ -D_\mu \delta\phi^\dagger D^\mu \phi - D_\mu \phi^\dagger D^\mu \delta\phi \right. \\
&\quad \left. - \lambda^2 \left( \phi^\dagger \phi - \frac{1}{2}v^2 \right) \left( \delta\phi^\dagger \phi + \phi^\dagger \delta\phi \right) \right] \sqrt{-g} d^4x \\
&= \hbar \int \delta\phi^\dagger \left[ D_\mu D^\mu \phi - \lambda^2 \left( \phi^\dagger \phi - \frac{1}{2}v^2 \right) \phi \right] \sqrt{-g} d^4x \\
&\quad + \delta\phi \hbar \left[ D_\mu D^\mu \phi^\dagger - \lambda^2 \left( \phi^\dagger \phi - \frac{1}{2}v^2 \right) \phi^\dagger \right] \sqrt{-g} d^4x
\end{aligned} \tag{4.9}$$

so the scalar field equation of motion is

$$-\frac{1}{2}D_\mu D^\mu \phi + \frac{1}{2}\lambda^2 \left( \phi^\dagger \phi - \frac{1}{2}v^2 \right) \phi = 0 \tag{4.10}$$

### 4.3 Spin(4)-symmetric energy-momentum tensors

The energy-momentum tensors of the Spin(4)-symmetric gauge and scalar fields are SO(4)-symmetric, so the energy-momentum tensors have the form

$$T_{\mu\nu} dx^\mu dx^\nu = \rho(T) a^2 dT^2 + p(T) a^2 ds_{S^3}^2 \tag{4.11}$$

of perfect fluids of density  $\rho$  and pressure  $p$ .

For the Spin(4)-symmetric gauge field, calculate the energy-momentum tensor (4.5) at the north-pole. Use equation (3.24) for  $F_{\mu\nu}$  at the north-pole.

$$\begin{aligned}
F_{0a}(T, \hat{N}) &= -\frac{1}{2} \partial_T b i^{-1} \sigma_a & F_{ab}(T, \hat{N}) &= \frac{1}{2} (b^2 - 1) \epsilon_{abc} i^{-1} \sigma_c \\
\text{tr}(F_{0\sigma} F_0^\sigma) &= a^{-2} \text{tr} \left[ \left( -\frac{1}{2} \partial_T b i^{-1} \sigma_a \right) \left( -\frac{1}{2} \partial_T b i^{-1} \sigma^a \right) \right] = -\frac{3}{2} a^{-2} (\partial_T b)^2 \\
\text{tr}(F_{a\sigma} F_b^\sigma) &= a^{-2} \text{tr}(-F_{a0} F_{b0} + F_{ac} F_b^c) \\
&= \frac{1}{4} a^{-2} (\partial_T b)^2 \text{tr}(\sigma_a \sigma_b) - \frac{1}{4} a^{-2} (b^2 - 1)^2 \epsilon_{acd} \epsilon_{bce} \text{tr}(\sigma_d \sigma_e) \\
&= \frac{1}{2} a^{-2} (\partial_T b)^2 \delta_{ab} - a^{-2} (b^2 - 1)^2 \delta_{ab} \\
\text{tr}(F_{\rho\sigma} F^{\rho\sigma}) &= a^{-2} \text{tr}(-F_{0\sigma} F_0^\sigma + F_{a\sigma} F^{b\sigma}) = 3a^{-4} [(\partial_T b)^2 - (b^2 - 1)^2]
\end{aligned} \tag{4.12}$$

So at the north-pole

$$\begin{aligned}
T_{00}^{\text{gauge}} &= \frac{\hbar}{g^2} \text{tr} \left( -2F_{0\sigma} F_0^\sigma + \frac{1}{2} g_{00} F_{\rho\sigma} F^{\rho\sigma} \right) = \frac{3\hbar}{g^2 a^2} \left[ \frac{1}{2} (\partial_T b)^2 + \frac{1}{2} (b^2 - 1)^2 \right] \\
&= \frac{3\hbar E_b}{g^2 a^2}
\end{aligned} \tag{4.13}$$

where

$$E_b = \frac{1}{2} (\partial_T b)^2 + \frac{1}{2} (b^2 - 1)^2 \tag{4.14}$$

The gauge energy-momentum tensor is traceless,  $g^{\mu\nu}T_{\mu\nu}^{\text{gauge}} = 0$ , so

$$\begin{aligned} T_{\mu\nu}^{\text{gauge}} dx^\mu dx^\nu &= \frac{3\hbar E_b}{g^2 a^2} \left( dT^2 + \frac{1}{3} ds_{S^3}^2 \right) \\ \rho_{\text{gauge}} &= \frac{3\hbar E_b}{g^2 a^4} \quad p_{\text{gauge}} = \frac{1}{3} \rho_{\text{gauge}} \end{aligned} \quad (4.15)$$

For the Spin(4)-symmetric scalar field  $\phi = 0$ , the energy-momentum tensor (4.6) is

$$\begin{aligned} T_{\mu\nu}^{\text{scalar}} &= \frac{\hbar \lambda^2 v^4}{8} (-g_{\mu\nu}) \\ T_{\mu\nu}^{\text{scalar}} dx^\mu dx^\nu &= \mathcal{E}_0 (a^2 dT^2 - a^2 ds_{S^3}^2) \\ \rho_{\text{scalar}} &= \mathcal{E}_0 \quad p_{\text{scalar}} = -\rho_{\text{scalar}} \quad \mathcal{E}_0 = \frac{\hbar \lambda^2 v^4}{8} \end{aligned} \quad (4.16)$$

#### 4.4 Spin(4)-symmetric gravitational equation of motion

The gravitational equation of motion (4.4)

$$G_{\mu\nu} = \kappa T_{\mu\nu}^{\text{gauge}} + \kappa T_{\mu\nu}^{\text{scalar}} \quad (4.17)$$

becomes two scalar equations on the Spin(4)-symmetric fields, one equation between the coefficients of  $dT^2$ , the other equation between the coefficients of  $ds_{S^3}^2$ . Combining formula (3.4) for the Einstein tensor,

$$G_{\mu\nu} dx^\mu dx^\nu = [3a^{-2}(\partial_T a)^2 + 3] dT^2 + [a^{-2}(\partial_T a)^2 - 2a^{-1}\partial_T^2 a - 1] ds_{S^3}^2 \quad (4.18)$$

with formulas (4.15) and (4.16) for the energy-momentum tensors

$$\begin{aligned} T_{\mu\nu}^{\text{gauge}} dx^\mu dx^\nu &= \rho_{\text{gauge}} a^2 \left( dT^2 + \frac{1}{3} ds_{S^3}^2 \right) \\ T_{\mu\nu}^{\text{scalar}} dx^\mu dx^\nu &= \rho_{\text{scalar}} a^2 (dT^2 - ds_{S^3}^2) \\ \rho_{\text{gauge}} &= \frac{3\hbar E_b}{g^2 a^4} \quad E_b = \frac{1}{2}(\partial_T b)^2 + \frac{1}{2}(b^2 - 1)^2 \\ \rho_{\text{scalar}} &= \mathcal{E}_0 \quad \mathcal{E}_0 = \frac{\hbar \lambda^2 v^4}{8} \end{aligned} \quad (4.19)$$

gives the gravitational equations of motion

$$\begin{aligned} 3a^{-2}(\partial_T a)^2 + 3 &= \kappa \rho_{\text{gauge}} a^2 + \kappa \rho_{\text{scalar}} a^2 \\ a^{-2}(\partial_T a)^2 - 2a^{-1}\partial_T^2 a - 1 &= \frac{1}{3} \kappa \rho_{\text{gauge}} a^2 - \kappa \rho_{\text{scalar}} a^2 \end{aligned} \quad (4.20)$$

Re-write the first equation as

$$\begin{aligned} \frac{1}{2}(\partial_T a)^2 + \frac{1}{2}a^2 - \frac{1}{6}\kappa \rho_{\text{scalar}} a^4 &= \frac{1}{6}\kappa \rho_{\text{gauge}} a^4 \\ \frac{1}{2}(\partial_T a)^2 + \frac{1}{2}a^2 - \frac{\kappa \mathcal{E}_0}{6}a^4 &= \frac{\kappa \hbar}{2g^2} E_b \end{aligned} \quad (4.21)$$

Re-write 1/3 times the first equation minus the second equation

$$2a^{-1}\partial_T^2 a + 2 = \frac{4}{3}\kappa\rho_{\text{scalar}}a^2$$

$$\partial_T^2 a + a - \frac{2}{3}\kappa\mathcal{E}_0 a^3 = 0$$
(4.22)

The gravitational equations of motion become

$$\frac{1}{2}(\partial_T a)^2 + \frac{1}{2}a^2 - \frac{\kappa\mathcal{E}_0}{6}a^4 = \frac{\kappa\hbar}{2g^2}E_b$$

$$\partial_T^2 a + a - \frac{2}{3}\kappa\mathcal{E}_0 a^3 = 0$$
(4.23)

In terms of the dimensionless scale factor  $\hat{a} = a/t_I$ ,

$$\frac{1}{2}(\partial_T \hat{a})^2 + \frac{1}{2}\hat{a}^2 - \frac{\kappa\mathcal{E}_0 t_I^2}{6}\hat{a}^4 = \frac{\kappa\hbar}{2g^2 t_I^2}E_b$$

$$\partial_T^2 \hat{a} + \hat{a} - \frac{2}{3}\kappa\mathcal{E}_0 t_I^2 \hat{a}^3 = 0$$
(4.24)

Use the definitions

$$\frac{\kappa\mathcal{E}_0 t_I^2}{3} = 1 \quad \epsilon_w^{-4} = \frac{2g^2 t_I^2}{\kappa\hbar}$$
(4.25)

the gravitational equations of motion are

$$E_{\hat{a}} = \epsilon_w^4 E_b$$

$$\partial_T^2 \hat{a} + \hat{a} - 2\hat{a}^3 = 0$$
(4.26)

where

$$E_{\hat{a}} = \frac{1}{2}(\partial_T \hat{a})^2 + \frac{1}{2}\hat{a}^2 - \frac{1}{2}\hat{a}^4$$
(4.27)

#### 4.5 Spin(4)-symmetric gauge and scalar equations of motion

For the Spin(4)-symmetric gauge field  $B = (1 + b)\gamma$  and scalar field  $\phi = 0$ , the scalar equation of motion (4.10) is trivially satisfied and the gauge equation of motion (4.8) is

$$D^\nu F_{\mu\nu} = 0$$
(4.28)

The latter is

$$0 = \delta \frac{1}{\hbar} S_{\text{gauge}} = \delta \frac{6\pi^2}{g^2} \int \frac{1}{2} [(\partial_T b)^2 - (b^2 - 1)^2] dT$$

$$= \delta \frac{6\pi^2}{g^2} \int [-\partial_T^2 b - (b^2 - 1)2b] \delta b dT$$
(4.29)

The gauge equation of motion (4.28) is the equation of motion

$$-\partial_T^2 b - (b^2 - 1)2b = 0$$
(4.30)

derived from the Spin(4)-symmetric action.

Alternatively, use the Hodge-\* operator

$$*F_{\mu\nu} = \frac{1}{2}\epsilon_{\mu\nu}^{\quad \nu\sigma} F_{\nu\sigma} \quad *^2 = -1$$
(4.31)

to re-write the equation of motion (4.28) as

$$D*F = d*F + [B, *F] = 0 \quad (4.32)$$

The curvature 2-form of the Spin(4)-symmetric gauge field  $B = (1 + b)\gamma$  is (3.23)

$$F = (\partial_T b) dT \wedge \gamma + (b^2 - 1)\gamma \wedge \gamma \quad (4.33)$$

At the north-pole,

$$\begin{aligned} *(dT \wedge d\hat{x}^a) &= \frac{1}{2} \epsilon_{abc} d\hat{x}^b \wedge d\hat{x}^c \\ *dT \wedge \gamma(\hat{N}) &= *dT \wedge \left( \frac{1}{2} d\hat{x}^a i\sigma_a \right) = \frac{1}{4} \epsilon_{abc} d\hat{x}^b \wedge d\hat{x}^c i\sigma_a = -\gamma \wedge \gamma(\hat{N}) \end{aligned} \quad (4.34)$$

so

$$*(dT \wedge \gamma) = -\gamma \wedge \gamma \quad *(\gamma \wedge \gamma) = dT \wedge \gamma \quad (4.35)$$

so, using the identity  $d\gamma = -2\gamma \wedge \gamma$ ,

$$\begin{aligned} *F &= (b^2 - 1)dT \wedge \gamma - (\partial_T b)\gamma \wedge \gamma \\ d*F &= 2(b^2 - 1)dT \wedge \gamma \wedge \gamma - (\partial_T^2 b)dT \wedge \gamma \wedge \gamma \\ [B, *F] &= (1 + b)(b^2 - 1)(\gamma \wedge dT \wedge \gamma - dT \wedge \gamma \wedge \gamma) \\ &= -2(1 + b)(b^2 - 1)dT \wedge \gamma \wedge \gamma \\ D*F &= (-\partial_T^2 b - 2b(b^2 - 1))dT \wedge \gamma \wedge \gamma \end{aligned} \quad (4.36)$$

So the equation of motion  $D*F = 0$  is the  $b$  oscillator equation of motion (4.30).

## 5 Numbers

### 5.1 Fundamental constants

From *2018 CODATA Recommended values of the fundamental constants of physics and chemistry*, NIST SP 959 (June 2019) [1]

Defining constants of the International System of Units (SI)

$$\begin{aligned} c &= 2.99792458 \times 10^8 \text{ ms}^{-1} \\ \hbar &= 1.054571817 \times 10^{-34} \text{ Js} \\ e &= 1.602176634 \times 10^{-19} \text{ C} \\ k_B &= 1.380649 \times 10^{-23} \text{ J K}^{-1} \end{aligned} \quad (5.1)$$

so

$$1 \text{ GeV} = 1.602176634 \times 10^{-10} \text{ J} = k_B (1.160452 \times 10^{13} \text{ K}) \quad (5.2)$$

Newtonian constant of gravitation

$$\begin{aligned} G &= 6.67430(15) \times 10^{-11} \text{ m}^3 \text{ kg}^{-1} \text{ s}^{-2} \\ \kappa &= 8\pi G = 1.10982 \times 10^{-61} \text{ s GeV}^{-1} c^5 \end{aligned} \quad (5.3)$$

## 5.2 Standard Model coupling constants

From Particle Data Group, *Review of Particle Physics 2018 and 2019 update* [2]

- Section 1. Physical Constants (p. 127)
- Section 10. Electroweak Model and Constraints on New Physics (p. 161)

$G_F$  and  $m_W$  are from Section 1 (p. 127).  $m_H$  is from the 2019 update.

$$\begin{aligned} G_F &= 1.1663787(6) \times 10^{-5} \text{ GeV}^{-2} \\ m_W &= 80.379(12) \text{ GeV} \\ m_H &= 125.10(14) \text{ GeV} \end{aligned} \tag{5.4}$$

In Section 10, the Higgs potential is written (in  $\hbar = 1$  units)

$$V(\phi) = -\mu^2 \phi^\dagger \phi + \frac{\lambda^2}{2} (\phi^\dagger \phi)^2 \tag{5.5}$$

(actually  $\mu^2$  is written there without the sign). This is the same as the Higgs potential in (1.1) up to the constant term. The couplings are related to measurements by

$$\langle \phi \rangle_{\text{vac}} = \frac{v}{\sqrt{2}} \quad m_H = \lambda \hbar v \quad m_W = \frac{1}{2} g \hbar v \quad \frac{G_F}{\sqrt{2}} = \frac{1}{2(\hbar v)^2} \tag{5.6}$$

which gives

$$\begin{aligned} \hbar v &= 2^{-\frac{1}{4}} G_F^{-\frac{1}{2}} = 246 \text{ GeV} \\ g &= \frac{2m_W}{\hbar v} = 0.653 \\ \lambda &= \frac{m_H}{\hbar v} = 0.508 \end{aligned} \tag{5.7}$$

## 5.3 Gravitational and weak time scales $t_{\text{grav}}$ , $t_W$

Define the gravitational time scale

$$t_{\text{grav}} = (\hbar \kappa)^{\frac{1}{2}} = (8\pi \hbar G)^{\frac{1}{2}} = (8\pi)^{\frac{1}{2}} t_P = 5.01 t_P = 2.70 \times 10^{-43} \text{ s} \tag{5.8}$$

where  $t_P = (\hbar G)^{\frac{1}{2}}$  is the Planck time.

Define the weak time scale

$$t_W = \frac{2}{gv} = \frac{\hbar}{m_W} = \frac{\hbar}{80.4 \text{ GeV}} = 8.19 \times 10^{-27} \text{ s} \tag{5.9}$$

## 5.4 The scalar field energy density $\mathcal{E}_0$

$$\frac{1}{\hbar} \mathcal{E}_0 = \frac{1}{8} \lambda^2 v^4 = \frac{1}{8} \lambda^2 \left( \frac{2}{g} \frac{1}{t_W} \right)^4 = \frac{2\lambda^2}{g^4} t_W^{-4} = 2.84 t_W^{-4} \tag{5.10}$$

## 5.5 Seesaw time scale $t_I$

$$\begin{aligned} t_I^2 &= \frac{3}{\kappa \mathcal{E}_0} = \frac{24}{\kappa \hbar \lambda^2 v^4} = \frac{1}{\kappa \hbar} \frac{3g^4}{2\lambda^2} t_W^4 = \frac{3g^4}{2\lambda^2} \frac{t_W^4}{t_{\text{grav}}^2} \\ t_I &= \sqrt{\frac{3}{2}} \frac{g^2}{\lambda} \frac{t_W^2}{t_{\text{grav}}} = 1.03 \frac{t_W^2}{t_{\text{grav}}} = 2.55 \times 10^{-10} \text{ s} = 7.64 \text{ cm} \end{aligned} \tag{5.11}$$

## 5.6 Seesaw ratio $\epsilon_w$

$$\epsilon_w^4 = \frac{\kappa \hbar}{2g^2 t_I^2} = \frac{\kappa \hbar}{2g^2} \frac{\kappa \hbar \lambda^2 v^4}{24} = \frac{\kappa^2 \hbar^2 \lambda^2 v^4}{48g^2} \quad \epsilon_w^2 = \frac{\kappa \hbar \lambda v^2}{4 \cdot 3^{1/2} g} \quad (5.12)$$

$$\epsilon_w = 3.39 \times 10^{-17} \quad (5.13)$$

$$\begin{aligned} \epsilon_w^4 &= \frac{\kappa \hbar}{2g^2 t_I^2} = \frac{1}{2g^2} \frac{t_{\text{grav}}^2}{t_I^2} & \epsilon_w &= \left( \frac{1}{2g^2} \right)^{\frac{1}{4}} \left( \frac{t_{\text{grav}}}{t_I} \right)^{\frac{1}{2}} = 1.04 \left( \frac{t_{\text{grav}}}{t_I} \right)^{\frac{1}{2}} \\ &= \frac{t_{\text{grav}}^2}{2g^2} \left( \frac{2\lambda^2 t_{\text{grav}}^2}{3g^4 t_W^4} \right) & \epsilon_w &= \left( \frac{\lambda^2}{3g^6} \right)^{\frac{1}{4}} \frac{t_{\text{grav}}}{t_W} = 1.03 \frac{t_{\text{grav}}}{t_W} \\ &= \left( \frac{1}{2g^2} \frac{t_{\text{grav}}^2}{t_I^2} \right)^2 \left( \frac{\lambda^2 t_{\text{grav}}^4}{3g^6 t_W^4} \right)^{-1} & \epsilon_w &= \left( \frac{3g^2}{4\lambda^2} \right)^{\frac{1}{4}} \frac{t_W}{t_I} = 1.05 \frac{t_W}{t_I} \end{aligned} \quad (5.14)$$

## 5.7 Units of action for the two oscillators

In the action (3.35) for the  $\hat{a}$  and  $b$  oscillators,

$$S = \frac{6\pi^2}{g^2} \hbar \int \left( -\epsilon_w^{-4} \left[ \frac{1}{2} (\partial_T \hat{a})^2 - V_{\hat{a}}(\hat{a}) \right] + \left[ \frac{1}{2} (\partial_T b)^2 - V_b(b) \right] \right) dT \quad (5.15)$$

The units of action for the  $b$  oscillator are

$$\hbar_b = \frac{6\pi^2}{g^2} \hbar = 139 \hbar \quad (5.16)$$

For the  $\hat{a}$  oscillator the units of action are

$$\hbar_{\hat{a}} = \frac{6\pi^2}{g^2} \epsilon_w^{-4} \hbar = 139 \epsilon_w^{-4} \hbar \quad (5.17)$$

## 6 Stability of $\phi = 0$

Expand the scalar field action (1.1)

$$\frac{1}{\hbar} S_{\text{scalar}} = \int \left[ -D_\mu \phi^\dagger D^\mu \phi - \frac{1}{2} \lambda^2 \left( \phi^\dagger \phi - \frac{1}{2} v^2 \right)^2 \right] \sqrt{-g} d^4 x \quad (6.1)$$

in powers of a perturbation  $\phi(x)$  around  $\phi = 0$ ,

$$\frac{1}{\hbar} S_{\text{scalar}}(\phi) = \frac{1}{\hbar} S_{\text{scalar}}(0) + \frac{1}{\hbar} S_{\text{scalar}}^{(2)}(\phi) + O(\phi^4) \quad (6.2)$$

$$\begin{aligned} \frac{1}{\hbar} S_{\text{scalar}}^{(2)} &= \int \left[ - (D_\mu \phi)^\dagger (D^\mu \phi) + \frac{1}{2} \lambda^2 v^2 \phi^\dagger \phi \right] \sqrt{-g} d^4 x \\ &= \int \left[ a^{-2} (\partial_T \phi)^\dagger (\partial_T \phi) - a^{-2} \mathcal{V}(\phi) \right] a^4 d^3 \hat{x} dT \end{aligned} \quad (6.3)$$

$$\mathcal{V}(\phi) = \hat{g}^{jk} (D_j \phi)^\dagger (D_k \phi) - a^2 \frac{1}{2} \lambda^2 v^2 \phi^\dagger \phi \quad (6.4)$$

where  $\hat{g}_{jk}$  is the metric of the unit 3-sphere,  $ds_{S^3}^2 = \hat{g}_{jk}(\hat{x})d\hat{x}^j d\hat{x}^k$  and  $D_0 = \partial_T$ ,  $D_k = \partial_k + B_k$  is the gauge covariant derivative, with  $B_k = (1+b)\gamma_k$ .

Stability of the  $\phi = 0$  solution is the condition that

$$0 \leq \int_{S^3} \left[ \hat{g}^{jk} (D_j \phi)^\dagger (D_k \phi) - a^2 \frac{1}{2} \lambda^2 v^2 \phi^\dagger \phi \right] d^3 \hat{x} \quad (6.5)$$

for all perturbations  $\phi(x)$ . Integrate by parts to write this

$$0 \leq \int_{S^3} \phi^\dagger \left[ \hat{g}^{jk} D_j^\dagger D_k - \frac{1}{2} a^2 \lambda^2 v^2 \right] \phi d^3 \hat{x} \quad (6.6)$$

so the stability condition is the operator condition

$$0 \leq \hat{g}^{jk} D_j^\dagger D_k - \frac{1}{2} a^2 \lambda^2 v^2 \quad (6.7)$$

Stability at time scales much longer than the  $b$  oscillation period is the time average condition

$$0 \leq \langle \hat{g}^{jk} D_j^\dagger D_k \rangle - \frac{1}{2} a^2 \lambda^2 v^2 \quad (6.8)$$

## 6.1 Dirac matrices and spinors on $S^3$

The Spin(4)-symmetric  $\mathfrak{su}(2)$ -valued 1-form  $\gamma$  defined by (2.3) and (2.30)

$$\begin{aligned} g_{\hat{x}} &= \hat{x}^4 \mathbf{1} + \hat{x}^a i^{-1} \sigma_a \\ \gamma(\hat{x}) &= -\frac{1}{2} (dg_{\hat{x}}) g_{\hat{x}}^{-1} = \frac{1}{2} g_{\hat{x}} dg_{\hat{x}}^\dagger \end{aligned} \quad (6.9)$$

At the north-pole  $\hat{N}$ ,

$$\gamma_a = \frac{1}{2} i \sigma_a \quad \gamma_a \gamma_b = -\frac{1}{4} \delta_{ab} - \frac{1}{4} i \epsilon_{abc} \sigma_c = -\frac{1}{4} \hat{g}_{ab} - \frac{1}{2} \epsilon_{ab}^c \gamma_c \quad (6.10)$$

so everywhere on  $S^3$

$$\gamma_j^\dagger = -\gamma_j \quad \gamma_j \gamma_k = -\frac{1}{4} \hat{g}_{jk} - \frac{1}{2} \epsilon_{jk}^i \gamma_i \quad \hat{g}^{jk} \gamma_j^\dagger \gamma_k = \hat{g}^{jk} (-\gamma_j) \gamma_k = \frac{3}{4} \mathbf{1} \quad (6.11)$$

so the matrices  $2i\gamma_j(\hat{x})$  can be interpreted as the Dirac matrices on  $S^3$ . The doublet scalar field  $\phi$  can be interpreted geometrically as a spinor on  $S^3$ .

## 6.2 Time-averaged stability

Write

$$D_k = D_k^0 + b\gamma_k \quad D_k^0 = \partial_k + \gamma_k \quad (6.12)$$

The  $b$  oscillations are symmetric in  $b \rightarrow -b$  so the time average  $\langle b \rangle = 0$  so

$$\begin{aligned} \langle \hat{g}^{jk} D_j^\dagger D_k \rangle &= \langle \hat{g}^{jk} (D_j^{0\dagger} + b\gamma_j^\dagger) (D_k^0 + b\gamma_k) \rangle \\ &= \hat{g}^{jk} D_j^{0\dagger} D_k^0 + \langle b^2 \rangle \hat{g}^{jk} \gamma_j^\dagger \gamma_k \\ &= \hat{g}^{jk} D_j^{0\dagger} D_k^0 + \frac{3}{4} \langle b^2 \rangle \end{aligned} \quad (6.13)$$

So the time-average stability condition is

$$0 \leq \hat{g}^{jk} D_j^{0\dagger} D_k^0 + \frac{3}{4} \langle b^2 \rangle - \frac{1}{2} a^2 \lambda^2 v^2 \quad (6.14)$$

### 6.3 Spinor covariant derivative

Let  $\nabla_j$  be the covariant derivative on vectors and tensors on the unit 3-sphere. Then

$$\nabla_j \gamma_k = \frac{1}{2} \partial_j g_{\hat{x}} \partial_k g_{\hat{x}}^\dagger + \frac{1}{2} g_{\hat{x}} \nabla_j \partial_k g_{\hat{x}}^\dagger \quad (6.15)$$

Calculate at the north-pole  $\hat{N} = (0, 0, 0, 1)$ ,

$$\partial_a \partial_b g_{\hat{x}}^\dagger(\hat{N}) = \partial_a \partial_b (\hat{x}^4 \mathbf{1} + \hat{x}^a i \sigma_a)_{/\hat{x}^a=0} = -\delta_{ab} \mathbf{1} \quad (6.16)$$

so everywhere on  $S^3$

$$\nabla_j \partial_k g_{\hat{x}}^\dagger = -\hat{g}_{jk} \quad (6.17)$$

Use this in (6.15) along with

$$\partial_j g_{\hat{x}} \partial_k g_{\hat{x}}^\dagger = (-2\gamma_j g_{\hat{x}})(2g_{\hat{x}}^{-1} \gamma_k) = -4\gamma_j \gamma_k = \hat{g}_{jk} + 2\epsilon_{jk}^i \gamma_i \quad (6.18)$$

to get

$$\nabla_j \gamma_k = \epsilon_{jk}^i \gamma_i \quad (6.19)$$

Now extend the gauge covariant derivative  $D_j^0 = \partial_j + \nabla_j$  to tensors with values in the fundamental bundle as

$$D_j^0 = \nabla_j + \gamma_j \quad (6.20)$$

Then

$$D_j^0 \gamma_k = \nabla_j \gamma_k + [\gamma_j, \gamma_k] = \epsilon_{jk}^i \gamma_i - \epsilon_{jk}^i \gamma_i = 0 \quad (6.21)$$

which is to say that the Dirac matrices are covariant constant under  $D_j^0$ . Therefore  $D_j^0$  is the spinor covariant derivative.

The curvature form of the spinor covariant derivative is

$$\begin{aligned} [D_j^0, D_k^0] &= [\nabla_j + \gamma_j, \nabla_k + \gamma_k] = [\nabla_j, \nabla_k] + \nabla_j \gamma_k - \nabla_k \gamma_j + [\gamma_j, \gamma_k] \\ &= [\nabla_j, \nabla_k] + \epsilon_{jk}^i \gamma_i \end{aligned} \quad (6.22)$$

The “spinors”  $\phi$  are functions with values in  $\mathbb{C}^2$ , so  $[\nabla_j, \nabla_k] \phi = 0$ , so

$$[D_j^0, D_k^0] \phi = \epsilon_{jk}^i \gamma_i \phi \quad (6.23)$$

### 6.4 Dirac operator

The Dirac operator on  $S^3$  is

$$\not{D} = 2\hat{g}^{jk} \gamma_j D_k^0 = 2\gamma^k D_k^0 \quad \not{D}^\dagger = \not{D} \quad (6.24)$$

Calculate  $\not{D}^2$  acting on “spinors”  $\phi$

$$\begin{aligned} \not{D}^2 &= 4\gamma^j D_j^0 \gamma^k D_k^0 = 4\gamma^j \gamma^k D_j^0 D_k^0 = (-\hat{g}^{jk} - 2\epsilon^{jki} \gamma_i) D_j^0 D_k^0 \\ &= \hat{g}^{jk} D_j^{0\dagger} D_k^0 - \epsilon^{jki} \gamma_i [D_j^0, D_k^0] = \hat{g}^{jk} D_j^{0\dagger} D_k^0 - \epsilon^{jki} \gamma_i \epsilon_{jk}^{i'} \gamma_{i'} \\ &= \hat{g}^{jk} D_j^{0\dagger} D_k^0 + 2\hat{g}^{ii'} \gamma_i \gamma_{i'} = \hat{g}^{jk} D_j^{0\dagger} D_k^0 + 2\hat{g}^{ii'} \hat{g}_{ii'} \\ &= \hat{g}^{jk} D_j^{0\dagger} D_k^0 + \frac{3}{2} \end{aligned} \quad (6.25)$$

then calculate the gauge laplacian acting on “spinors”  $\phi$

$$\begin{aligned}
\hat{g}^{jk} D_j^\dagger D_k &= -\hat{g}^{jk} (D_j^0 + b\gamma_j)(D_k^0 + b\gamma_k) = -\hat{g}^{jk} D_j^0 D_k^0 - 2b\gamma^k D_k^0 - b^2 \hat{g}^{jk} \gamma_j \gamma_k \\
&= \not{D}^2 - \frac{3}{2} - b\not{D} + \frac{3}{4}b^2 \\
&= \left(\not{D} - \frac{1}{2}b\right)^2 - \frac{3}{2} + \frac{1}{2}b^2
\end{aligned} \tag{6.26}$$

so there is a bound

$$0 \leq \left(\not{D} - \frac{1}{2}b\right)^2 - \frac{3}{2} + \frac{1}{2}b^2 \tag{6.27}$$

Minimize the rhs wrt  $b$

$$2\left(\not{D} - \frac{1}{2}b\right)\left(-\frac{1}{2}\right) + b = 0 \quad b = \frac{2}{3}\not{D} \tag{6.28}$$

to get the bound

$$0 \leq \left(\not{D} - \frac{1}{2}\frac{2}{3}\not{D}\right)^2 - \frac{3}{2} + \frac{1}{2}\left(\frac{2}{3}\not{D}\right)^2 = \frac{2}{3}\not{D}^2 - \frac{3}{2} \tag{6.29}$$

or

$$\left(\frac{3}{2}\right)^2 \leq \not{D}^2 \tag{6.30}$$

Equality,  $\not{D} = \pm 3/2$ , requires  $b = \pm 1$ . Equality is equivalent to  $\hat{g}^{jk} D_j^\dagger D_k = 0$  which is equivalent to  $D_k = 0$ . For  $b = -1$ ,

$$D_k \phi = (\partial_k + \gamma_k + b\gamma_k)\phi = \partial_k \phi \tag{6.31}$$

so the zero mode of  $D_k$  is  $\phi = \phi_0$  a constant. When  $b = 1$ ,

$$D_k \phi = (\partial_k + 2\gamma_k)\phi = (\partial_k + g_{\hat{x}} dg_{\hat{x}}^\dagger)\phi = g_{\hat{x}} \partial_k (g_{\hat{x}}^{-1} \phi) \tag{6.32}$$

so the zero mode of  $D_k$  is then  $\phi = g_{\hat{x}} \phi_0$  with  $\phi_0$  constant.

## 6.5 Parity operator

Let the parity operator  $P \in O(4)$  be

$$P: (\hat{x}^i, \hat{x}^4) \mapsto (-\hat{x}^i, \hat{x}^4) \tag{6.33}$$

so

$$g_{P\hat{x}} = g_{\hat{x}}^{-1} \tag{6.34}$$

Let  $P$  act on the fundamental  $SU(2)$  bundle by

$$P\phi(\hat{x}) = g_{\hat{x}}\phi(P\hat{x}) \tag{6.35}$$

$P$  has the following properties

$$\begin{aligned}
P^2\phi(\hat{x}) &= P(g_{\hat{x}}\phi(P\hat{x})) = g_{\hat{x}}g_{P\hat{x}}\phi(P^2\hat{x}) = \phi(\hat{x}) \\
P\gamma P^{-1} &= P\frac{1}{2}g_{\hat{x}}d(g_{\hat{x}}^{-1})P^{-1} = \frac{1}{2}g_{\hat{x}}g_{P\hat{x}}d(g_{P\hat{x}}^{-1})g_{\hat{x}}^{-1} = \frac{1}{2}(dg_{\hat{x}})g_{\hat{x}}^{-1} = -\gamma \\
PD^0P^{-1} &= P(d + \gamma)P^{-1} = g_{\hat{x}}dg_{\hat{x}}^{-1} - \gamma = d + g_{\hat{x}}d(g_{\hat{x}}^{-1}) - \gamma = d + \gamma = D^0
\end{aligned} \tag{6.36}$$

which are

$$P^2 = 1 \quad P\gamma P^{-1} = -\gamma \quad PD^0 P^{-1} = D^0 \quad (6.37)$$

These imply

$$P\mathcal{D}P^{-1} = -\mathcal{D} \quad (6.38)$$

and

$$PDP^{-1} = P(D^0 + b\gamma)P^{-1} = D^0 - b\gamma \quad (6.39)$$

so the SU(2) gauge field  $b(T)$  is parity-odd.

## 6.6 Time-averaged stability (II)

Combine the identity (6.25) with the bound (6.30)

$$\left(\frac{3}{2}\right)^2 \leq \mathcal{D}^2 = \hat{g}^{jk} D_j^{0\dagger} D_k^0 + \frac{3}{2} \quad (6.40)$$

to get the bound

$$\frac{3}{4} \leq \hat{g}^{jk} D_j^{0\dagger} D_k^0 \quad (6.41)$$

with the lower bound realized on the constants  $\phi = \phi_0$  and on their gauge transforms  $\phi = P\phi_0 = g_{\hat{x}}\phi_0$ . So the time-averaged stability condition (6.14) is

$$0 \leq \frac{3}{4} + \frac{3}{4}\langle b^2 \rangle - \frac{1}{2}a^2\lambda^2v^2 \quad (6.42)$$

The stability condition is first violated when  $a$  reaches  $a_{\text{EW}}$  given by equality in (6.42)

$$\frac{2}{3}\lambda^2v^2a_{\text{EW}}^2 = 1 + \langle b^2 \rangle \quad (6.43)$$

When  $a$  is slightly greater than  $a_{\text{EW}}$ , the zero modes  $\phi = \phi_0$  and their gauge transforms  $\phi = P\phi_0$  are the only unstable modes. The other modes of  $\phi(x)$  become unstable at larger values of  $a$ .

## 7 Solution of the $b$ oscillator by an elliptic function

### 7.1 Reparametrize $T$ and $b$

The energy equation for the  $b$  oscillator is

$$\frac{1}{2} \left( \frac{db}{dT} \right)^2 + \frac{1}{2}(b^2 - 1)^2 = E_b \quad (7.1)$$

$b$  oscillates between  $\pm b_{\text{max}}$  where

$$\frac{1}{2}(b_{\text{max}}^2 - 1)^2 = E_b \quad b_{\text{max}}^2 - 1 = (2E_b)^{\frac{1}{2}} \quad (7.2)$$

Write the energy equation

$$\left( \frac{db}{dT} \right)^2 = 2E_b - (b^2 - 1)^2 = (b_{\text{max}}^2 - 1)^2 - (b^2 - 1)^2 = (b_{\text{max}}^2 - b^2)(b_{\text{max}}^2 - 2 + b^2) \quad (7.3)$$

Change variables from  $T$  and  $b(T)$  to  $z$  and  $y(z)$

$$T = \epsilon_b z \quad b = b_{\max} y \quad (7.4)$$

with  $\epsilon_b$  to be determined. Now the energy equation is

$$\begin{aligned} \frac{b_{\max}^2}{\epsilon_b^2} \left( \frac{dy}{dz} \right)^2 &= (b_{\max}^2 - b_{\max}^2 y^2)(b_{\max}^2 - 2 + b_{\max}^2 y^2) \\ \left( \frac{dy}{dz} \right)^2 &= (1 - y^2)(\epsilon_b^2 b_{\max}^2 - 2\epsilon_b^2 + \epsilon_b^2 b_{\max}^2 y^2) \end{aligned} \quad (7.5)$$

which is

$$\left( \frac{dy}{dz} \right)^2 = (1 - y^2)(1 - k^2 + k^2 y^2) \quad (7.6)$$

for

$$1 - k^2 = \epsilon_b^2 b_{\max}^2 - 2\epsilon_b^2 \quad k^2 = \epsilon_b^2 b_{\max}^2 \quad (7.7)$$

The sum of these last two equations gives

$$1 = 2\epsilon_b^2 b_{\max}^2 - 2\epsilon_b^2 = 2\epsilon_b^2 (b_{\max}^2 - 1) = 2\epsilon_b^2 (2E_b)^{\frac{1}{2}} \quad \epsilon_b = (8E_b)^{-\frac{1}{4}} \quad (7.8)$$

The difference of the two equations gives

$$2k^2 - 1 = 2\epsilon_b^2 \quad k^2 = \frac{1}{2} + \epsilon_b^{-2} \quad (7.9)$$

## 7.2 The Jacobi elliptic function $\text{cn}(z, k)$

The energy equation (7.6)

$$\left( \frac{dy}{dz} \right)^2 = (1 - y^2)(1 - k^2 + k^2 y^2) \quad (7.10)$$

is solved by the Jacobi elliptic function [3, 4]

$$y = \text{cn}(z, k) \quad (7.11)$$

by integrating

$$\begin{aligned} \frac{dy}{dz} &= -\sqrt{(1 - y^2)(1 - k^2 + k^2 y^2)} \quad dz = \frac{-dy}{\sqrt{(1 - y^2)(1 - k^2 + k^2 y^2)}} \\ z &= \int_{\text{cn}(z, k)}^1 \frac{dy}{\sqrt{(1 - y^2)(1 - k^2 + k^2 y^2)}} \end{aligned} \quad (7.12)$$

## 7.3 Properties of the Jacobi elliptic functions

The Jacobi elliptic functions [3, 4] are  $\text{sn}(z, k)$ ,  $\text{cn}(z, k)$ ,  $\text{dn}(z, k)$ .

Differential equations:

| $y$               | $\left( \frac{dy}{dz} \right)^2 =$ | $\frac{d^2 y}{dz^2} =$    |
|-------------------|------------------------------------|---------------------------|
| $\text{sn}(z, k)$ | $(1 - y^2)(1 - k^2 y^2)$           | $-(1 + k^2)y + 2k^2 y^3$  |
| $\text{cn}(z, k)$ | $(1 - y^2)(1 - k^2 + k^2 y^2)$     | $-(1 - 2k^2)y - 2k^2 y^3$ |
| $\text{dn}(z, k)$ | $(y^2 - 1)(1 - k^2 - y^2)$         | $(2 - k^2)y - 2y^3$       |

(7.13)

Derivatives:

$$\operatorname{sn}' = \operatorname{cn} \operatorname{dn} \quad \operatorname{cn}' = -\operatorname{sn} \operatorname{dn} \quad \operatorname{dn}' = -k^2 \operatorname{sn} \operatorname{cn} \quad (7.14)$$

Reflections:

$$\operatorname{sn}(-z) = -\operatorname{sn}(z) \quad \operatorname{cn}(-z) = \operatorname{cn}(z) \quad \operatorname{dn}(-z) = \operatorname{dn}(z) \quad (7.15)$$

Algebraic relations:

$$\operatorname{sn}^2 + \operatorname{cn}^2 = 1 \quad k^2 \operatorname{sn}^2 + \operatorname{dn}^2 = 1 \quad k^2 \operatorname{cn}^2 = \operatorname{dn}^2 + k^2 - 1 \quad (7.16)$$

A doubling identity:

$$\left( \frac{\operatorname{sn} \operatorname{dn}}{\operatorname{cn}} \right)^2 (z, k) = \frac{1 - \operatorname{cn}(2z, k)}{1 + \operatorname{cn}(2z, k)} \quad (7.17)$$

In the following,

$$k^2 + k'^2 = 1 \quad K = K(k) \quad K' = K(k') \quad (7.18)$$

where  $K(k)$  is the complete elliptic integral of the first kind.

Poles and zeros:

|    | pole  | zero      |                 |
|----|-------|-----------|-----------------|
| sn | $iK'$ | 0         | $+ 2mK + 2inK'$ |
| cn | $iK'$ | $K$       |                 |
| dn | $iK'$ | $K + iK'$ |                 |

(7.19)

Half-periods:

$$\begin{aligned} \operatorname{sn}(z + 2Km + 2K'm'i) &= (-1)^m \operatorname{sn}(z) \\ \operatorname{cn}(z + 2Km + 2K'm'i) &= (-1)^{m+m'} \operatorname{cn}(z) \\ \operatorname{dn}(z + 2Km + 2K'm'i) &= (-1)^{m'} \operatorname{dn}(z) \end{aligned} \quad (7.20)$$

Quarter periods:

$$\begin{aligned} \operatorname{sn}(z + K) &= \frac{\operatorname{cn}}{\operatorname{dn}}(z) & \operatorname{sn}(z + iK') &= \frac{1}{k}(z) \frac{1}{\operatorname{sn}}(z) \\ \operatorname{cn}(z + K) &= -k' \frac{\operatorname{sn}}{\operatorname{dn}}(z) & \operatorname{cn}(z + iK') &= \frac{1}{ik} \frac{\operatorname{dn}}{\operatorname{sn}}(z) \\ \operatorname{dn}(z + K) &= k' \frac{1}{\operatorname{dn}}(z) & \operatorname{dn}(z + iK') &= \frac{1}{i} \frac{\operatorname{cn}}{\operatorname{sn}}(z) \end{aligned} \quad (7.21)$$

Residues and Taylor expansions:

$$\begin{aligned} \operatorname{sn}(z) &= z - (1 + k^2) \frac{z^3}{3!} + \cdots & \operatorname{sn}(iK' + z) &= \frac{1/k}{z} + \cdots \\ \operatorname{cn}(z) &= 1 - \frac{z^2}{2!} + \cdots & \operatorname{cn}(iK' + z) &= \frac{-i/k}{z} + \cdots \\ \operatorname{dn}(z) &= 1 - k^2 \frac{z^2}{2!} + \cdots & \operatorname{dn}(iK' + z) &= \frac{-i}{z} + \cdots \end{aligned} \quad (7.22)$$

## 7.4 Complete elliptic integral of first kind $K(k)$ , $K'(k)$

From (7.12) the real quarter-period  $K$  of  $\text{cn}(z, k)$  is

$$K(k) = \int_0^1 \frac{dy}{\sqrt{(1-y^2)(1-k^2+k^2y^2)}} \quad (7.23)$$

Changing variable  $y = \cos \theta$ , this is

$$K = \int_0^{\frac{\pi}{2}} \frac{d\theta}{\sqrt{(1-k^2 \sin^2 \theta)}} \quad (7.24)$$

the complete elliptic integral of first kind.

The imaginary quarter-period is

$$\begin{aligned} iK' &= \int_1^\infty \frac{dy}{\sqrt{(1-y^2)(1-k^2+k^2y^2)}} = \int_0^1 \frac{d(y^{-1})}{\sqrt{(1-y^{-2})(1-k^2+k^2y^{-2})}} \\ &= \int_0^1 \frac{idy}{\sqrt{(1-y^2)[k^2+(1-k^2)y^2]}} \\ &= iK(k') \end{aligned} \quad (7.25)$$

where

$$k^2 + k'^2 = 1 \quad (7.26)$$

## 7.5 $K(1/\sqrt{2})$

For  $k^2 = k'^2 = \frac{1}{2}$ ,

$$\begin{aligned} K(1/\sqrt{2}) &= \int_0^1 \frac{dy}{\sqrt{(1-y^2)(1-\frac{1}{2}+\frac{1}{2}y^2)}} = \int_0^1 \frac{\sqrt{2} dy}{\sqrt{1-y^4}} = \int_0^1 \frac{\sqrt{2} d(s^{1/4})}{\sqrt{1-s}} \\ &= \frac{\sqrt{2}}{4} \int_0^1 s^{-3/4}(1-s)^{-1/2} ds \end{aligned} \quad (7.27)$$

The beta function is

$$B(x, y) = \int_0^1 t^{x-1}(1-t)^{y-1} dt = \frac{\Gamma(x)\Gamma(y)}{\Gamma(x+y)} \quad (7.28)$$

so

$$K(1/\sqrt{2}) = \frac{\sqrt{2}}{4} B(1/4, 1/2) = \frac{\sqrt{2}}{4} \frac{\Gamma(1/4)\Gamma(1/2)}{\Gamma(3/4)} \quad (7.29)$$

Use

$$\Gamma(z)\Gamma(1-z) = \frac{\pi}{\sin \pi z} \quad \Gamma(1/2)^2 = \pi \quad \Gamma(1/4)\Gamma(3/4) = \sqrt{2}\pi \quad (7.30)$$

to get

$$K(1/\sqrt{2}) = K'(1/\sqrt{2}) = \frac{\Gamma(1/4)^2}{4\pi^{1/2}} = 1.854075 \dots \quad (7.31)$$

## 7.6 $\langle \text{cn}^2 \rangle$ for $k = 1/\sqrt{2}$

The time average  $\langle \text{cn}^2 \rangle$  of  $\text{cn}(z, k)$  over a real cycle can, by the symmetries, be calculated over a quarter-cycle

$$\langle \text{cn}^2 \rangle = \frac{1}{K} \int_0^K \text{cn}^2(z, k) dz = \frac{1}{K} \int_0^1 \frac{y^2 dy}{\sqrt{(1-y^2)(1-k^2+k^2y^2)}} \quad (7.32)$$

For  $k = 1/\sqrt{2}$ ,

$$\begin{aligned} \langle \text{cn}^2 \rangle &= \frac{1}{K} \int_0^1 \frac{\sqrt{2} y^2 dy}{\sqrt{1-y^4}} = \frac{1}{K} \sqrt{2} \int_0^1 \frac{s^{1/2} d(s^{1/4})}{\sqrt{1-s}} \\ &= \frac{1}{K} \frac{\sqrt{2}}{4} \int_0^1 s^{-1/4} (1-s)^{-1/2} ds = \frac{1}{K} \frac{\sqrt{2}}{4} B(3/4, 1/2) \\ &= \frac{1}{K} \frac{\sqrt{2}}{4} \frac{\Gamma(3/4)\Gamma(1/2)}{\Gamma(5/4)} = \frac{1}{K} \frac{\sqrt{2}}{4} \frac{\sqrt{2}\pi}{\Gamma(1/4)} \frac{\pi^{1/2}}{\frac{1}{4}\Gamma(1/4)} = \frac{1}{K} \frac{2\pi^{3/2}}{\Gamma(1/4)^2} \\ &= \frac{\pi}{2} \frac{1}{K^2} = 0.45694658 \dots \end{aligned} \quad (7.33)$$

## 7.7 $\langle \text{cn}^2 \rangle$ for general $k$

For general  $k$

$$\begin{aligned} K \langle \text{cn}^2 \rangle &= \int_0^1 \frac{y^2 dy}{\sqrt{(1-y^2)(1-k^2+k^2y^2)}} \\ (1-k^2)K + k^2 K \langle \text{cn}^2 \rangle &= \int_0^1 \frac{(1-k^2+k^2y^2) dy}{\sqrt{(1-y^2)(1-k^2+k^2y^2)}} \\ &= \int_0^1 \sqrt{\frac{1-k^2+k^2y^2}{1-y^2}} dy = \int_0^{\pi/2} \sqrt{1-k^2 \sin^2 \theta} d\theta \end{aligned} \quad (7.34)$$

which is the complete elliptic integral of the second kind

$$E(k) = \int_0^{\pi/2} \sqrt{1-k^2 \sin^2 \theta} d\theta \quad (7.35)$$

so

$$\begin{aligned} (1-k^2)K + k^2 K \langle \text{cn}^2 \rangle &= E \\ [3, 5.134] \quad \langle \text{cn}^2 \rangle &= \frac{E - (1-k^2)K}{k^2 K} \end{aligned} \quad (7.36)$$

The identity

$$[3, 8.122] \quad EK' + E'K - KK' = \frac{\pi}{2} \quad (7.37)$$

gives a check for  $k = 1/\sqrt{2}$ , where  $K = K'$ ,  $E = E'$ ,

$$2EK - K^2 = \frac{\pi}{2} \quad E = \frac{\pi}{4K} + \frac{1}{2}K \quad \langle \text{cn}^2 \rangle = \frac{E - \frac{1}{2}K}{\frac{1}{2}K} = \frac{\frac{\pi}{4K}}{\frac{1}{2}K} = \frac{\pi}{2K^2} \quad (7.38)$$

## 8 Cosmological temperature

For  $E_b \gg 1$

$$k = 1/\sqrt{2} \quad b = b_{\max} \operatorname{cn}(z, k) \quad b_{\max} = (2E_b)^{1/4} \quad (8.1)$$

$$\langle b^2 \rangle = \langle b_{\max}^2 \operatorname{cn}^2 \rangle = (2E_b)^{1/2} \frac{\pi}{2K^2} \quad (8.2)$$

Equation (6.43) for  $a_{\text{EW}}$

$$\frac{2}{3} \lambda^2 v^2 a_{\text{EW}}^2 = 1 + \langle b^2 \rangle \quad (8.3)$$

becomes, since  $\langle b^2 \rangle \gg 1$ ,

$$\frac{2}{3} \lambda^2 v^2 a_{\text{EW}}^2 = (2E_b)^{1/2} \frac{\pi}{2K^2} \quad (8.4)$$

or

$$\begin{aligned} a_{\text{EW}}^2 &= \frac{1}{\lambda^2 v^2} \frac{3}{2} (2E_b)^{1/2} \frac{\pi}{2K^2} = \frac{3\pi}{4K^2} (2E_b)^{1/2} \frac{1}{\lambda^2 v^2} \\ a_{\text{EW}} &= \frac{(3\pi)^{1/2}}{2K} (2E_b)^{1/4} \frac{1}{\lambda v} = \frac{(3\pi)^{1/2}}{2K} \frac{1}{4^{1/4} \epsilon_b} \frac{\hbar}{m_{\text{H}}} = \frac{(6\pi)^{1/2}}{4K \epsilon_b} \frac{\hbar}{m_{\text{H}}} \end{aligned} \quad (8.5)$$

Co-moving time  $t$  is obtained by integrating

$$dt = a(T) dT \quad (8.6)$$

$b(T)$  is periodic in imaginary proper time  $T$  with period  $K\epsilon_b$ . This is very small compared to the time scale  $E_a^{-1/4}$  on which  $a(T)$  changes by a factor of  $\epsilon_w \approx 10^{-17}$ . So  $b$  is periodic in imaginary co-moving time with period  $K\epsilon_b a$ . The inverse temperature is the period in imaginary co-moving time

$$\frac{\hbar}{k_{\text{B}} T_{\text{SU}(2)}} = 4K\epsilon_b a \quad k_{\text{B}} T_{\text{SU}(2)} = \frac{\hbar}{4K\epsilon_b a} = \frac{m_{\text{H}}}{(6\pi)^{1/2}} \frac{a_{\text{EW}}}{a} = 28.8 \text{ GeV} \frac{a_{\text{EW}}}{a} \quad (8.7)$$

$$k_{\text{B}} T_{\text{EW}} = 28.8 \text{ GeV} \quad T_{\text{EW}} = 3.34 \times 10^{14} \text{ K} \quad (8.8)$$

## 9 Solution of the $\hat{a}$ oscillator

### 9.1 Solution for $\hat{a}$ in co-moving time

Co-moving time  $t$  is given by

$$dt = a(T) dT \quad a^2(-dT^2 + ds_{\text{S}^3}^2) = -dt^2 + a^2 ds_{\text{S}^3}^2 \quad (9.1)$$

Define the dimensionless co-moving time  $\hat{t}$

$$t = t_{\text{I}} \hat{t} \quad d\hat{t} = \hat{a}(T) dT \quad (9.2)$$

The  $\hat{a}$  energy equation (4.27)

$$\frac{1}{2} (\partial_T \hat{a})^2 + \frac{1}{2} \hat{a}^2 - \frac{1}{2} \hat{a}^4 = E_{\hat{a}} \quad (9.3)$$

becomes

$$\frac{1}{2} \hat{a}^2 (\partial_{\hat{t}} \hat{a})^2 + \frac{1}{2} \hat{a}^2 - \frac{1}{2} \hat{a}^4 = E_{\hat{a}} \quad (9.4)$$

Change variables,

$$\hat{a} = (2E_{\hat{a}})^{1/4} u \quad \epsilon_a = (2E_{\hat{a}})^{-1/4} \quad (9.5)$$

The energy equation now becomes

$$\begin{aligned}
(2E_{\hat{a}})\frac{1}{2}u^2(\partial_{\hat{t}}u)^2 + (2E_{\hat{a}})^{1/2}\frac{1}{2}u^2 - (2E_{\hat{a}})\frac{1}{2}u^4 &= E_{\hat{a}} \\
u^2(\partial_{\hat{t}}u)^2 + (2E_{\hat{a}})^{-1/2}u^2 - u^4 &= 1 \\
u^2(\partial_{\hat{t}}u)^2 + \epsilon_a^2u^2 - u^4 &= 1
\end{aligned} \tag{9.6}$$

Change variable again

$$\begin{aligned}
u^2 = w + \frac{1}{2}\epsilon_a^2 \quad \frac{1}{4}(\partial_{\hat{t}}w)^2 + \epsilon_a^2\left(w + \frac{1}{2}\epsilon_a^2\right) - \left(w + \frac{1}{2}\epsilon_a^2\right)^2 &= 1 \\
\frac{1}{4}(\partial_{\hat{t}}w)^2 - w^2 &= 1 - \frac{1}{4}\epsilon_a^4
\end{aligned} \tag{9.7}$$

Take the  $\hat{t}$  derivative

$$\begin{aligned}
\frac{1}{2}(\partial_{\hat{t}}w)\partial_{\hat{t}}^2w - 2w(\partial_{\hat{t}}w) &= 0 \\
\partial_{\hat{t}}^2w - 4w &= 0 \\
w &= A_1e^{2\hat{t}} + A_2e^{-2\hat{t}}
\end{aligned} \tag{9.8}$$

Fix the origin in  $\hat{t}$  by

$$u(0) = 0 \quad A_1 + A_2 = -\frac{1}{2}\epsilon_a^2 \tag{9.9}$$

Substitute in (9.7)

$$\begin{aligned}
\left(A_1e^{2\hat{t}} - A_2e^{-2\hat{t}}\right)^2 - \left(A_1e^{2\hat{t}} + A_2e^{-2\hat{t}}\right)^2 &= 1 - \frac{1}{4}\epsilon_a^4 \\
-4A_1A_2 &= 1 - \frac{1}{4}\epsilon_a^4 \\
(A_1 - A_2)^2 = (A_1 + A_2)^2 - 4A_1A_2 &= \frac{1}{4}\epsilon_a^4 + 1 - \frac{1}{4}\epsilon_a^4 = 1 \quad A_1 - A_2 = \pm 1
\end{aligned} \tag{9.10}$$

$$\begin{aligned}
A_1 &= \pm\frac{1}{2} - \frac{1}{4}\epsilon_a^2 \quad A_2 = \mp\frac{1}{2} - \frac{1}{4}\epsilon_a^2 \\
u^2 &= \left(\pm\frac{1}{2} - \frac{1}{4}\epsilon_a^2\right)e^{2\hat{t}} + \left(\mp\frac{1}{2} - \frac{1}{4}\epsilon_a^2\right)e^{-2\hat{t}} + \frac{1}{2}\epsilon_a^2
\end{aligned} \tag{9.11}$$

Use the solution with  $u$  increasing with time

$$u^2 = \left(\frac{1}{2} - \frac{1}{4}\epsilon_a^2\right)e^{2\hat{t}} + \left(-\frac{1}{2} - \frac{1}{4}\epsilon_a^2\right)e^{-2\hat{t}} + \frac{1}{2}\epsilon_a^2 \tag{9.12}$$

Define

$$k_a^2 = \frac{1}{2} + \frac{1}{4}\epsilon_a^2 \tag{9.13}$$

Then

$$u^2 = (1 - k_a^2)e^{2\hat{t}} - k_a^2e^{-2\hat{t}} + 2k_a^2 - 1 = (e^{2\hat{t}} - 1)(1 - k_a^2 + k_a^2e^{-2\hat{t}}) \tag{9.14}$$

So the solution for  $\hat{a}$  is

$$\begin{aligned}
\epsilon_a &= (2E_{\hat{a}})^{-1/4} \quad k_a^2 = \frac{1}{2} + \frac{1}{4}\epsilon_a^2 \\
\hat{a} &= (2E_{\hat{a}})^{1/4}u \quad u = \sqrt{(e^{2\hat{t}} - 1)(1 - k_a^2 + k_a^2e^{-2\hat{t}})}
\end{aligned} \tag{9.15}$$

Proper time is given by

$$\begin{aligned}\frac{d\hat{t}}{dT} &= \hat{a} = \epsilon_a^{-1} \sqrt{(e^{2\hat{t}} - 1) (1 - k_a^2 + k_a^2 e^{-2\hat{t}})} \\ \frac{e^{-\hat{t}}}{\epsilon_a^{-1}} \frac{d\hat{t}}{dT} &= \sqrt{(1 - e^{-2\hat{t}}) (1 - k_a^2 + k_a^2 e^{-2\hat{t}})} \\ T &= \epsilon_a z_a \quad y_a = e^{-\hat{t}}\end{aligned}\tag{9.16}$$

$$-\frac{dy_a}{dz_a} = \sqrt{(1 - y_a^2) (1 - k_a^2 + k_a^2 y_a^2)}$$

$$y_a = \text{cn}(z_a, k_a)$$

so the relation between co-moving and proper time is

$$e^{-\hat{t}} = \text{cn}(z_a, k_a) \quad T = \epsilon_a z_a\tag{9.17}$$

Since  $E_{\hat{a}} \gg 1$ ,

$$k_a^2 = \frac{1}{2} \quad \hat{a} = (2E_{\hat{a}})^{1/4} u \quad u = \sqrt{(e^{2\hat{t}} - 1) \left(\frac{1}{2} + \frac{1}{2} e^{-2\hat{t}}\right)} = \sqrt{\sinh(2\hat{t})}\tag{9.18}$$

$$K_a = K(1/\sqrt{2}) = \frac{\Gamma(1/4)^2}{4\pi^{1/2}} = 1.854075 \dots$$

The ratio of the  $b$  oscillation time scale to the expansion time scale is

$$\frac{\epsilon_b}{\epsilon_a} = \frac{(8E_b)^{-1/4}}{(2E_{\hat{a}})^{-1/4}} = \frac{\epsilon_w}{\sqrt{2}} = 2.40 \times 10^{-17}\tag{9.19}$$

## 9.2 $\hat{a}_{\text{EW}}$

As  $t$  goes from 0 to  $\infty$ ,

| $t$             | $\hat{t}$             | $u$             | $\hat{a}$             | $a$             | $e^{-\hat{t}} = \text{cn}(z_a, k_a)$ | $T = \epsilon_a z_a$ |
|-----------------|-----------------------|-----------------|-----------------------|-----------------|--------------------------------------|----------------------|
| 0               | 0                     | 0               | 0                     | 0               | 1                                    | 0                    |
| $\vdots$        | $\vdots$              | $\vdots$        | $\vdots$              | $\vdots$        | $\vdots$                             | $\vdots$             |
| $t_{\text{EW}}$ | $\hat{t}_{\text{EW}}$ | $u_{\text{EW}}$ | $\hat{a}_{\text{EW}}$ | $a_{\text{EW}}$ | $e^{-\hat{t}_{\text{EW}}}$           | $T_{\text{EW}}$      |
| $\vdots$        | $\vdots$              | $\vdots$        | $\vdots$              | $\vdots$        | $\vdots$                             | $\vdots$             |
| $\infty$        | $\infty$              | $\infty$        | $\infty$              | $\infty$        | 0                                    | $K_a \epsilon_a$     |

(9.20)

Here  $T_{\text{EW}}$  is the proper time at the onset of the electroweak transition, not the temperature. Equation (8.5) gives

$$a_{\text{EW}} = \frac{(3\pi)^{1/2} (2E_b)^{1/4}}{2K} \frac{1}{\lambda v} \quad a_{\text{EW}}^2 = \frac{3\pi}{4K^2} \frac{(2E_b)^{1/4}}{\lambda^2 v^2}\tag{9.21}$$

Recall (5.11), (5.12)

$$\begin{aligned}a^2 &= t_1^2 \hat{a}^2 \quad t_1^2 = \frac{24}{\kappa \hbar \lambda^2 v^4} = (2.55 \times 10^{-10} \text{ s})^2 \\ E_b &= \epsilon_w^{-4} E_{\hat{a}} \quad \epsilon_w^2 = \frac{\kappa \hbar \lambda v^2}{4 \cdot 3^{1/2} g} = (3.39 \times 10^{-17})^2\end{aligned}\tag{9.22}$$

So the dimensionless scale factor  $\hat{a}_{\text{EW}}$  at the onset of the electroweak transition is

$$\begin{aligned}
\hat{a}_{\text{EW}}^2 &= t_{\text{I}}^{-2} a_{\text{EW}}^2 = \frac{\kappa \hbar \lambda^2 v^4}{24} \frac{3\pi}{4K^2} \frac{(2E_b)^{1/4}}{\lambda^2 v^2} = \frac{\pi}{32K^2} \kappa \hbar v^2 (2\epsilon_{\text{w}}^{-4} E_{\hat{a}})^{1/2} \\
&= \frac{\pi}{32K^2} \kappa \hbar v^2 (2E_{\hat{a}})^{1/2} \frac{4 \cdot 3^{1/2} g}{\kappa \hbar \lambda v^2} \\
&= \frac{3^{1/2} \pi}{8K^2} \frac{g}{\lambda} (2E_{\hat{a}})^{1/2} = \frac{3^{1/2} \pi}{8K^2} \frac{2m_W}{m_{\text{H}}} (2E_{\hat{a}})^{1/2} = 0.254 (2E_{\hat{a}})^{1/2}
\end{aligned} \tag{9.23}$$

In terms of the solution (9.18) for  $\hat{a}(t)$ ,

$$\begin{aligned}
u_{\text{EW}}^2 &= (2E_{\hat{a}})^{-1/2} \hat{a}_{\text{EW}}^2 = \frac{3^{1/2} \pi}{4K^2} \frac{m_W}{m_{\text{H}}} = 0.254 \\
\hat{t}_{\text{EW}} &= \frac{1}{2} \text{arcsinh}(u_{\text{EW}}^2) = \frac{1}{2} \text{arcsinh}(0.254) = 0.126 \\
t_{\text{EW}} &= \hat{t}_{\text{EW}} t_{\text{I}} = 0.126 t_{\text{I}} = 3.21 \times 10^{-11} \text{ s} \\
T_{\text{EW}} &= \text{arccn}(e^{-\hat{t}_{\text{EW}}}, k_a) \epsilon_a = 0.501 \epsilon_a
\end{aligned} \tag{9.24}$$

### 9.3 The function $u(z, k)$

This subsection is not used in the paper. In this subsection, write  $z$  in place of  $z_a$  and  $k$  in place of  $k_a$ .

The function  $u(z, k)$  given by

$$u = \sqrt{\left(e^{2\hat{t}} - 1\right) \left(1 - k^2 + k^2 e^{-2\hat{t}}\right)} \quad e^{-\hat{t}} = \text{cn}(z, k) \tag{9.25}$$

has some nice properties. The identities (7.16) for the Jacobi elliptic functions give

$$\begin{aligned}
1 - e^{-2\hat{t}} &= 1 - \text{cn}^2(z, k) = \text{sn}^2(z, k) \\
1 - k^2 + k^2 e^{-2\hat{t}} &= 1 - k^2 + k^2 \text{cn}^2(z, k) = \text{dn}^2(z, k)
\end{aligned} \tag{9.26}$$

so

$$u(z, k) = \frac{\text{sn dn}}{\text{cn}}(z, k) \tag{9.27}$$

Then identity (7.17) gives

$$u(z, k) = \sqrt{\frac{1 - \text{cn}(2z, k)}{1 + \text{cn}(2z, k)}} \tag{9.28}$$

and by identity (7.14)

$$u(z, k) = \frac{d}{dz} [-\ln \text{cn}(z, k)] = \frac{d\hat{t}}{dz} \tag{9.29}$$

(which returns to the starting point  $\hat{a} = d\hat{t}/dT$ .)

So  $u(z, k)$  has the equivalent forms

$$u(z, k) = \frac{\text{sn dn}}{\text{cn}}(z, k) = \sqrt{\frac{1 - \text{cn}(2z, k)}{1 + \text{cn}(2z, k)}} = \frac{d}{dz} [-\ln \text{cn}(z, k)] \tag{9.30}$$

From the quarter-period identities (7.21),  $u(z) = u(z, k)$  satisfies

$$u(z + K) = \frac{-1}{u(z)} \quad u(z + iK') = \frac{1}{u(z)} \quad u(-z) = -u(z) \quad (9.31)$$

from which

$$u(z) = u(z + 2K) = u(z + 2iK') = -u(z + K + iK') \quad (9.32)$$

From the expansions (7.22),

$$u(z - K) = \frac{-1}{z} + O(z) \quad u(z) = z + O(z^3) \quad u(z + K) = \frac{-1}{z} + O(z) \quad (9.33)$$

Equation (7.19) lists the poles and zeros of  $\text{cn}$ ,  $\text{sn}$ , and  $\text{dn}$ ,

|             | pole  | zero      |                 |
|-------------|-------|-----------|-----------------|
| $\text{sn}$ | $iK'$ | $0$       | $+ 2mK + 2inK'$ |
| $\text{cn}$ | $iK'$ | $K$       |                 |
| $\text{dn}$ | $iK'$ | $K + iK'$ |                 |

(9.34)

So the zeros and poles of  $u = \text{sn dn} / \text{cn}$  are the lattice points  $nK + n'iK'$ , for all integers  $n, n'$ . The zeros are at the lattice points with  $n + n'$  even, the poles at the points with  $n + n'$  odd. In particular,  $u(z)$  has poles at  $z = \pm K$  and  $\pm iK'$  and zeros at  $z = 0$  and  $K + iK'$ .

$u(z, k)$  satisfies the differential equation

$$\left( \frac{du}{dz} \right)^2 = (u^2 + 1)^2 - 4k^2 u^2 \quad (9.35)$$

derived by

$$\begin{aligned} u^2 &= \frac{\text{sn}^2 \text{dn}^2}{\text{cn}^2} = \frac{(1 - \text{cn}^2)(k^2 \text{cn}^2 - k^2 + 1)}{\text{cn}^2} = -k^2 \text{cn}^2 + 2k^2 - 1 - (k^2 - 1) \text{cn}^{-2} \\ 2uu' &= [-2k^2 \text{cn} + 2(k^2 - 1) \text{cn}^{-3}] (-\text{sn dn}) \\ u' &= k^2 \text{cn}^2 - (k^2 - 1) \text{cn}^{-2} \\ u' - u^2 - 1 &= 2k^2(\text{cn}^2 - 1) \quad u' + u^2 + 1 = 2k^2 + 2(-k^2 + 1) \text{cn}^{-2} \\ (u' - u^2 - 1)(u' + u^2 + 1) &= -4k^2 u^2 \\ u'^2 &= (u^2 + 1)^2 - 4k^2 u^2 \end{aligned} \quad (9.36)$$

#### 9.4 Direct solution of the $\hat{a}$ oscillator by an elliptic function

This subsection is not used in the paper. The solution for  $\hat{a}(T)$  is found directly, without going to co-moving time.

Change variables from  $T$  and  $\hat{a}(T)$  to  $z_a$  and  $u(z_a)$

$$T = \epsilon_a z_a \quad \hat{a} = \epsilon_a^{-1} u \quad \epsilon_a = (2E_{\hat{a}})^{-1/4} \quad (9.37)$$

The energy equation (4.27)

$$E_{\hat{a}} = \frac{1}{2} (\partial_T \hat{a})^2 + \frac{1}{2} \hat{a}^2 - \frac{1}{2} \hat{a}^4 \quad (9.38)$$

becomes

$$\begin{aligned}
(\partial_T \hat{a})^2 &= 2E_{\hat{a}} - \hat{a}^2 + \hat{a}^4 \\
\epsilon_a^{-2} \epsilon_a^{-2} (\partial_{z_a} u)^2 &= \epsilon_a^{-4} - \epsilon_a^{-2} u^2 + \epsilon_a^{-4} u^4 \\
(\partial_{z_a} u)^2 &= 1 - \epsilon_a^2 u^2 + u^4
\end{aligned} \tag{9.39}$$

Define

$$k_a^2 = \frac{1}{2} + \frac{1}{4} \epsilon_a^2 \tag{9.40}$$

so

$$\begin{aligned}
(\partial_{z_a} u)^2 &= 1 - 4 \left( k_a^2 - \frac{1}{2} \right) u^2 + u^4 \\
&= (1 + u^2)^2 - 4k_a^2 u^2
\end{aligned} \tag{9.41}$$

Let

$$u = \sqrt{\frac{1 - y_a}{1 + y_a}} \quad u^2 = \frac{1 - y_a}{1 + y_a} = \frac{2}{1 + y_a} - 1 \tag{9.42}$$

Then

$$\begin{aligned}
\left[ \frac{d(u^2)}{dz_a} \right]^2 &= \left( 2u \frac{du}{dz_a} \right)^2 \\
\left[ \frac{-2}{(1 + y_a)^2} \frac{dy_a}{dz_a} \right]^2 &= 4u^2 [(1 + u^2)^2 - 4k_a^2 u^2] \\
\frac{4}{(1 + y_a)^4} \left( \frac{dy_a}{dz_a} \right)^2 &= 4 \left( \frac{1 - y_a}{1 + y_a} \right) \left[ \frac{4}{(1 + y_a)^2} - 4k_a^2 \left( \frac{1 - y_a}{1 + y_a} \right) \right] \\
\frac{1}{4} \left( \frac{dy_a}{dz_a} \right)^2 &= (1 + y_a)^4 \left( \frac{1 - y_a}{1 + y_a} \right) \left[ \frac{1}{(1 + y_a)^2} - k_a^2 \left( \frac{1 - y_a}{1 + y_a} \right) \right] \\
\frac{1}{4} \left( \frac{dy_a}{dz_a} \right)^2 &= (1 + y_a)(1 - y_a) [1 - k_a^2(1 + y_a)(1 - y_a)] \\
\frac{1}{4} \left( \frac{dy_a}{dz_a} \right)^2 &= (1 - y_a^2) (1 - k_a^2 + k_a^2 y_a^2)
\end{aligned} \tag{9.43}$$

So

$$y_a = \text{cn}(2z_a, k_a) \quad u(z_a, k_a) = \sqrt{\frac{1 - \text{cn}(2z_a, k_a)}{1 + \text{cn}(2z_a, k_a)}} \tag{9.44}$$

$$\begin{aligned}
a &= (2E_{\hat{a}})^{1/4} u(z_a, k_a) & T &= \epsilon_a z_a & \epsilon_a &= (2E_{\hat{a}})^{-1/4} & k_a^2 &= \frac{1}{2} + \frac{1}{4} \epsilon_a^2 \\
K_a &= K(k_a) & K'_a &= K'(ka)
\end{aligned} \tag{9.45}$$

# Numerical calculations for "Origins of Cosmological Temperature"

This SageMath notebook performs numerical calculations for the paper *Origins of Cosmological Temperature* and the supplemental note *Calculations for "Origins of Cosmological Temperature"*.

It makes graphs of the two anharmonic potentials and does some arithmetic.

Section headings are as in the supplemental note.

## 3.5 Action in dimensionless variables

```
In [1]: ah = var('ah')
E_ah = 0.15
ah_lim=1.08
ah_plot=plot((1/2)*(ah^2-ah^4), (ah,-ah_lim,ah_lim),aspect_ratio=12)
ah_plot+=text(r'$E_{\hat{a}}$', (-1.35,E_ah),fontsize=8)
ah_plot+=text(r'$0$', (-1.3,0),fontsize=6)
ah_plot+=text(r'$\frac{1}{8}$', (-1.32,0.125),fontsize=6,aspect_ratio=1)
ah_plot+=text(r'$0$', (0,-0.006),fontsize=6,aspect_ratio=1)
ah_plot+=text(r'$1$', (0.95,-0.006),fontsize=6,aspect_ratio=1)
ah_plot+=text(r'$-1$', (-1.0,-0.006),fontsize=6,aspect_ratio=1)
ah_plot+=text(r'$V_{\hat{a}}=\frac{1}{2}(\hat{a}^2-\hat{a}^4)$', (0,-0.04),fontsize=12)
ah_plot+= plot(0.125,(ah,-1.25,1.25),linestyle=":")
ah_plot+= plot(0,(ah,-1.25,1.25),linestyle=":")
ah_plot+= plot(E_ah,(ah,-1.25,1.25),linestyle=":")
ah_plot+=arrow((1.11,-0.08),(1.13,-0.08-.02),width=.5,arrowsize=1.5)
ah_plot+=arrow((-1.13,-0.08-.02),(-1.11,-0.08),width=.5,arrowsize=1.5)
ah_plot+=arrow((0.97,1/16),(1.00,1/16-.02),width=.5,arrowsize=1.5)
ah_plot+=arrow((-1.00,1/16-.02),(-0.97,1/16),width=.5,arrowsize=1.5)
ah_plot+=arrow((-0.34,1/16),(-0.27,1/16-.017),width=.5,arrowsize=1.5)
ah_plot+=arrow((0.27,1/16-.017),(0.34,1/16),width=.5,arrowsize=1.5)
ah_plot.save('plot_ah.pdf',dpi=200,axes=False)
show(ah_plot,axes=False,dpi=200,figsize=[3.2,2.4])
```

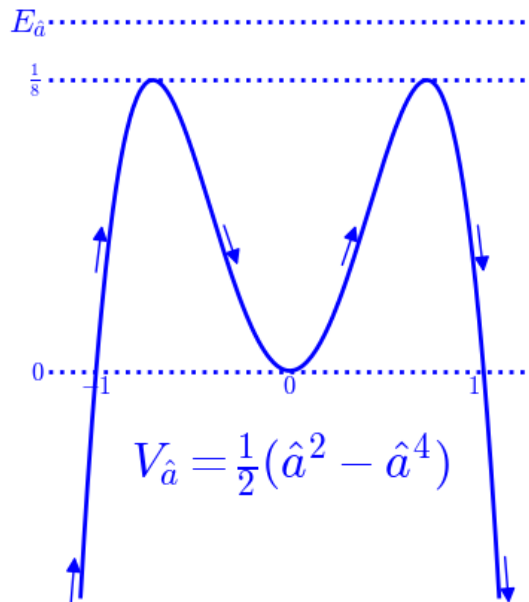

```
In [2]: b = var('b')
E_b = 12
b_plot=plot((1/2)*(b^2-1)^2, (b,-2.5,2.5),aspect_ratio=.5)
b_plot+=text(r'$E_b$',(-3.1,E_b),fontsize=10)
b_plot+=text(r'$0$',(-3.0,0),fontsize=6)
b_plot+=text(r'$V_b=\frac{1}{2}(b^2-1)^2$',(0,E_b/2),fontsize=12)
b_plot+=text(r'$b$',(0,-1),fontsize=12)
b_plot+= plot(0,(b,-2.7,2.7),linestyle=":")
b_plot+= plot(E_b,(b,-2.7,2.7),linestyle=":")
b_plot+=text(r'$1$',(1.0,-0.4),fontsize=6)
b_plot+=text(r'$0$',(0.0,-0.4),fontsize=6)
b_plot+=text(r'$-1$',(-1.0,-0.4),fontsize=6)
b_plot+=arrow((-1.97,E_b-2),(-1.9,E_b-4),width=.5,arrowsize=2)
b_plot.save('plot_b.pdf',dpi=200,axes=False)
show(b_plot,axes=False,dpi=200,figsize=[3.2,2.4])
```

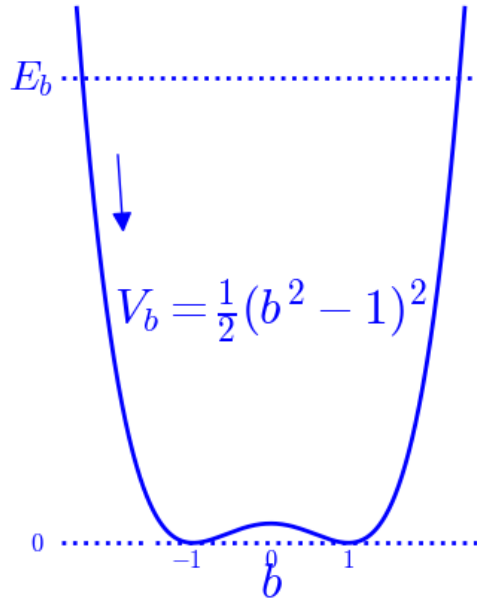

## 5.1 Fundamental constants

```
In [3]: %display latex
LE = lambda latex_string: LatexExpr(latex_string);
```

declare units as variables

```
In [4]: s = var('s', domain='positive'); assume(s,'real');
GeV = var('GeV', domain='positive'); assume(GeV,'real');
J = var('J', domain='positive'); assume(J,'real');
m = var('m', domain='positive'); assume(m,'real');
meters = var('meters', domain='positive'); assume(meters,'real');
kg = var('kg', domain='positive'); assume(kg,'real');
K = var('K', domain='positive'); assume(K,'real');
C = var('C', domain='positive'); assume(C,'real');
```

fundamental constants from NIST 2018

```
In [5]: c = 299792458 * meters * s^(-1);
e_charge = 1.602176634 * 10^(-19) * C;
hbar = 1.054571817*10^(-34)*J*s;
kB = 1.380649*10^(-23)*J*K^(-1);
G = 6.67430*10^(-11)*m^3*kg^(-1)* s^(-2);
kappa = N(8*pi)*G;
#
pretty_print(LE(r" c ="),c);
pretty_print(LE(r" e ="),e_charge);
pretty_print(LE(r"\hbar ="),hbar);
pretty_print(LE(r"k_{B} ="),kB);
pretty_print(LE(r"G ="),G);
pretty_print(LE(r"\kappa ="),kappa);
```

$$c = \frac{299792458 \text{ meters}}{s}$$

$$e = (1.60217663400000 \times 10^{-19}) \text{ C}$$

$$\hbar = (1.05457181700000 \times 10^{-34}) \text{ Js}$$

$$k_B = \frac{(1.38064900000000 \times 10^{-23}) \text{ J}}{K}$$

$$G = \frac{(6.67430000000000 \times 10^{-11}) \text{ m}^3}{\text{kgs}^2}$$

$$\kappa = \frac{(1.67743454782835 \times 10^{-9}) \text{ m}^3}{\text{kgs}^2}$$

use c=1 units with unit of energy = GeV

```
In [6]: m = c^(-1)*meters;
J = e_charge^(-1) * C * 10^(-9) * GeV
kg = J*s^2*m^(-2)
def conv(*args):
    return [arg.subs(m=m,kg=kg,J=J) for arg in args]
[hbar,kB,G,kappa] = conv(hbar,kB,G,kappa)
pretty_print(LE(r"\hbar ="),hbar);
pretty_print(LE(r"k_{B} ="),kB);
pretty_print(LE(r"G ="),G);
pretty_print(LE(r"\kappa ="),kappa);
```

$$\hbar = (6.58211956547607 \times 10^{-25}) \text{ GeVs}$$

$$k_B = \frac{(8.61733326214518 \times 10^{-14}) \text{ GeV}}{K}$$

$$G = \frac{(4.41583261432942 \times 10^{-63}) \text{ s}}{\text{GeV}}$$

$$\kappa = \frac{(1.10981978405276 \times 10^{-61}) \text{ s}}{\text{GeV}}$$

## 5.2 Standard Model coupling constants from PDG (2018, 2019)

```
In [7]: GFermi = 1.1663787*10^(-5)*GeV^(-2);
mW = 80.379*GeV;
mH = 125.10*GeV;
#
pretty_print(LE(r"G_F ="),GFermi);
pretty_print(LE(r"m_W ="),mW);
pretty_print(LE(r"m_H ="),mH);
```

$$G_F = \frac{0.0000116637870000000}{\text{GeV}^2}$$

$$m_W = 80.3790000000000 \text{ GeV}$$

$$m_H = 125.100000000000 \text{ GeV}$$

```
In [8]: hbar_v = N(2^(-1/4))*GFermi^(-1/2)
pretty_print(LE(r"\hbar v = 2^{-1/4} G_F^{-1/2}="),hbar_v)
v = hbar_v/hbar
pretty_print(LE(r"v ^{-1} ="),1/v);
g = 2*mW/hbar_v;
pretty_print(LE(r"g = \frac{2 m_W}{\hbar v}="),g)
lambdaH = mH/hbar_v;
pretty_print(LE(r"\lambda = \frac{m_H}{\hbar v}="),lambdaH)
```

$$\hbar v = 2^{-1/4} G_F^{-1/2} = 246.219650794137 \text{ GeV}$$

$$v^{-1} = (2.67327142421274 \times 10^{-27}) \text{ s}$$

$$g = \frac{2m_W}{\hbar v} = 0.652904833068782$$

$$\lambda = \frac{m_H}{\hbar v} = 0.508082923505546$$

### 5.3 Gravitational and weak time scales $t_{\text{grav}}, t_W$

```
In [9]: tgrav = sqrt(kappa*hbar);
pretty_print(LE(r"t_{\mathrm{grav}} = (\hbar\kappa)^{1/2}=\backslash(8\pi)^{1/2} t_P="),N((8*pi)^(1/2)),LE(r"t_P\backslash="),tgrav)
```

$$t_{\text{grav}} = (\hbar\kappa)^{1/2} = (8\pi)^{1/2} t_P = 5.01325654926200 t_P \\ = (2.70277015574135 \times 10^{-43}) \text{ s}$$

```
In [10]: tW = hbar/mW;
pretty_print(LE(r"t_{\mathrm{W}}=\frac{\hbar}{m_W}="),tW)
```

$$t_W = \frac{\hbar}{m_W} = (8.18885475743176 \times 10^{-27}) \text{ s}$$

### 5.4 The scalar field energy density $\mathcal{E}_0$

```
In [11]: E0 = hbar*lambdaH^2*v^4/8;
ratio1 = tW^4*E0/hbar;
pretty_print(LE(r"\frac{1}{\hbar}\mathcal{E}_0="),\ratio1,LE(r"\: t_{\mathrm{W}}^{-4}"))
```

$$\frac{1}{\hbar} \mathcal{E}_0 = 2.84118595562545 t_W^{-4}$$

### 5.5 Seesaw time scale $t_I$

```
In [12]: tI = (3/(kappa*E0))^(1/2);
ratio2 = tI*tgrav/tW^2;
pretty_print(LE(r"t_I="),ratio2,LE(r"\:\frac{t_{\mathrm{W}}^2}{t_{\mathrm{grav}}}\}),\LE(r"="),tI)
```

$$t_I = 1.02756853595816 \frac{t_W^2}{t_{\text{grav}}} = (2.54945892615748 \times 10^{-10}) \text{ s}$$

```
In [13]: ratio12 = N(sqrt(3/2))*g^2/lambdaH;
pretty_print(LE(r"\sqrt{\frac{3}{2}}\frac{g^2}{\lambda}="),ratio12);
```

$$\sqrt{\frac{3}{2}} \frac{g^2}{\lambda} = 1.02756853595816$$

```
In [14]: tI*c;
pretty_print(LE(r"t_I c="),tI*c);
```

$$t_I c = 0.0764308558042792 \text{ meters}$$

## 5.6 Seesaw ratio $\epsilon_W$

```
In [15]: epsilonW = (kappa*hbar/(2*g^2*tI^2))^(1/4);
pretty_print(LA(r"\epsilon_W="),epsilonW)
```

$$\epsilon_W = 3.38842679174089 \times 10^{-17}$$

```
In [16]: ratio3 = epsilonW*tW/tgrav;
ratio4 = epsilonW*tI/tW;
ratio34 = sqrt(ratio3*ratio4);
pretty_print(LA(r"\epsilon_W="),ratio34,
              LA(r"\left(\frac{t_{\mathrm{grav}}}{t_I}\right)^{1/2}"))
pretty_print(LA(r"\epsilon_W="),ratio3,
              LA(r"\frac{t_{\mathrm{grav}}}{t_{\mathrm{W}}}))
pretty_print(LA(r"\epsilon_W="),ratio4,
              LA(r"\frac{t_{\mathrm{W}}}{t_I}"))
```

$$\epsilon_W = 1.04068084127939 \left( \frac{t_{\mathrm{grav}}}{t_I} \right)^{1/2}$$

$$\epsilon_W = 1.02662576744880 \frac{t_{\mathrm{grav}}}{t_W}$$

$$\epsilon_W = 1.05492833683428 \frac{t_W}{t_I}$$

```
In [17]: ratio134=(2*g^2)^(-1/4);
pretty_print(LA(r"\left(\frac{1}{2g^2}\right)^{1/4}="),ratio134)
```

$$\left( \frac{1}{2g^2} \right)^{1/4} = 1.04068084127939$$

```
In [18]: ratio13=(lambdaH^2/(3*g^6))^(1/4);
pretty_print(LA(r"\left(\frac{\lambda^2}{3g^6}\right)^{1/4}="),ratio13)
```

$$\left( \frac{\lambda^2}{3g^6} \right)^{1/4} = 1.02662576744880$$

```
In [19]: ratio14=((3*g^2)/(4*lambdaH^2))^(1/4);
pretty_print(LA(r"\left(\frac{3g^2}{4\lambda^2}\right)^{1/4}="),ratio14)
```

$$\left( \frac{3g^2}{4\lambda^2} \right)^{1/4} = 1.05492833683428$$

## 5.7 Units of action for the two oscillators

```
In [20]: ratio5=6*N(pi)^2/g^2;
pretty_print(LA(r"\frac{6\pi^2}{g^2}="),ratio5)
```

$$\frac{6\pi^2}{g^2} = 138.915667118982$$

## 7.5 $K(1/\sqrt{2})$

```
In [21]: K = N(gamma(1/4)^2/(4*pi^(1/2)));
pretty_print(LA(r"K(1/sqrt{2}) = \frac{\Gamma(1/4)^2}{4 \pi^{1/2}}="),K)
```

$$K(1/\sqrt{2}) = \frac{\Gamma(1/4)^2}{4\pi^{1/2}} = 1.85407467730137$$

## 7.6 $\langle \text{cn}^2 \rangle$ for $k = 1/\sqrt{2}$

```
In [22]: cn2ave = N(pi/2)/K^2;
pretty_print(LE(r"\langle \mathrm{cn}^2 \rangle=\frac{2}{\pi^2}\frac{1}{K^2}="),cn2ave)
```

$$\langle \text{cn}^2 \rangle = \frac{2}{\pi^2} \frac{1}{K^2} = 0.456946581044464$$

## 8. Cosmological temperature

```
In [23]: kT = mH/N((6*pi)^(1/2));
pretty_print(LE(r"k_B T="),kT)
```

$$k_B T = 28.8142120659094 \text{ GeV}$$

```
In [24]: pretty_print(LE(r"T="),kT/kB)
```

$$T = 3.34375046077032 \times 10^{14} \text{ K}$$

## 9.1 Solution for $\hat{a}$ in co-moving time

```
In [25]: pretty_print(LE(r"\frac{\epsilon_W}{\sqrt{2}}="),epsilonW/N(sqrt(2)))
```

$$\frac{\epsilon_W}{\sqrt{2}} = 2.39597956199416 \times 10^{-17}$$

## 9.2 $\hat{a}_{EW}$

```
In [26]: ratio6 =N(3^(1/2)*pi/(8*K^2))*(2*mW/mH);
pretty_print(LE(r"\hat{a}_{\mathrm{EW}}="),\
LE(r"\frac{3^{1/2}\pi}{8 K^2}\frac{2m_W}{m_H}(2 E_{\hat{a}})^{1/2}="),\
ratio6,LE(r"\:(2 E_{\hat{a}})^{1/2}"))
```

$$\hat{a}_{EW}^2 = \frac{3^{1/2} \pi}{8 K^2} \frac{2 m_W}{m_H} (2 E_{\hat{a}})^{1/2} = 0.254261938075174 (2 E_{\hat{a}})^{1/2}$$

```
In [27]: pretty_print(LE(r"\hat{a}_{\mathrm{EW}}="),\
sqrt(ratio6),\
LE(r"\:(2 E_{\hat{a}})^{1/4}"))
```

$$\hat{a}_{EW} = 0.504243927157457 (2 E_{\hat{a}})^{1/4}$$

```
In [28]: thatEW = asinh(ratio6)/2;
pretty_print(LE(r"\hat{t}_{\mathrm{EW}}="),thatEW)
```

$$\hat{t}_{EW} = 0.125799532989201$$

```
In [29]: tEW = thatEW * tI;
pretty_print(LE(r"t_{\mathrm{EW}}="),tEW)
```

$$t_{EW} = (3.20720742285761 \times 10^{-11}) \text{ s}$$

```
In [30]: TEW = inverse_jacobi('cn', e^(-thatEW), 0.5);
pretty_print(LE(r"T_{\mathrm{EW}}="),TEW,LE(r"\;\epsilon_a"))
```

$$T_{EW} = 0.501068706214232 \epsilon_a$$

## References

- [1] E. Tiesinga *et al.*, “The 2018 CODATA Recommended Values of the Fundamental Physical Constants.” <http://physics.nist.gov/constants>.
- [2] **Particle Data Group** Collaboration, M. Tanabashi *et al.*, “Review of Particle Physics,” *Phys. Rev. D* **98** no. 3, (2018) 030001. and 2019 update, <http://pdg.lbl.gov/>, Sections 1 and 10.
- [3] I. Gradshteyn, A. Jeffrey, and I. Ryzhik, *Table of Integrals, Series, and Products*. Academic Press, 1996. Sections 8.11, 8.14, 8.15.
- [4] F. W. J. Olver *et al.*, “*NIST Digital Library of Mathematical Functions*.” Release 1.0.26 of 2020-03-15, <http://dlmf.nist.gov/>. Chapter 22 and section 19.2.
